# Supplementary material for: Exploring Weight Importance and Hessian Bias in Model Pruning
Source: arXiv:2006.10903 source file (2020-06-19)
Supplement: Supplementary file 1 [file appendix_deter.tex]

\section{Proofs for Gradient Descent Results}
\subsection{Proof of Theorem \ref{early stop cor}}
First, we have the following helper lemma.
\begin{lemma}[Noise Robustness of Features]\label{lem robust} Let $\bt,\ab\in\R^p$ be an arbitrary vectors and $\bb$ be a vector satisfying $\tin{\bb}\leq \Gamma/2$. Then
\[
|\conf{\bt,\bt+\ab+\bb}|\leq \frac{4\tn{\ab}^2}{\Gamma^2}.
\]
\end{lemma}
%\[
%|\supg{\bt+\ab+\bb}-\supg{\bt}|+|\supg{\bt}-\supg{\bt+\ab+\bb}|\leq \frac{4\tn{\ab}^2}{\Gamma^2}.
%\]
\begin{proof} Define the sets $S_1=\supt{\bt+\ab+\bb}-\suph{\bt}$ and $S_2=\supt{\bt}-\suph{\bt+\ab+\bb}$. $i\in S_1$ implies that $|\theta_i|<\Gamma/2$ and
\[
|\theta_i+a_i+b_i|\geq 3\Gamma/2\implies |a_i|\geq 3\Gamma/2-|\theta_i|-|b_i|> \Gamma/2. 
\]
$i\in S_2$ implies that $|\theta_i|\l\geq 3\Gamma/2$ and 
\[
|\theta_i+a_i+b_i|< \Gamma/2\implies |\theta_i+a_i|< \Gamma\implies |a_i|>\Gamma/2. 
\]
Hence if $i\in\conf{\bt,\bt+\ab+\bb}$, $|a_i|\geq \Gamma/2$. This implies that $\sqrt{|S_1|+|S_2|}\Gamma/2\leq \tn{\ab}$.
\end{proof}

Theorem \ref{early stop cor} is an immediate corollary of the following Theorem \ref{early stop main} after simplifying $\tn{\La_{1:r}^{-1/2}\z'_{1:r}}\leq \tn{\z'_{1:r}}/\sqrt{\la_r}$ and ${\sum_{i=1}^r\la_i^{-1}}\leq {r/\la_r}$.
\begin{theorem}[Feature Robustness with Early-stopping - General]\label{early stop main} Let $\X$ have singular value decomposition $\X=\Ub\sqrt{\La}\V^T=\sum_{i=1}^n\sqrt{\la_i}\ub_i\vb_i^T$. Define the triple $(\X',\y',\z')=(\Ub^T\X,\Ub^T\y,\Ub^T\z)$. Set learning rate $\eta\leq \frac{1}{\|\X\|^2}=\frac{1}{\la_1}$. Starting from $\bt_0=0$, after $T$ iterations, we have 
\[
\bt_T=\sum_{i=1}^n (1-(1-\eta\la_i)^{T})\frac{y'_i}{\sqrt{\la_i}} \vb_i.
\]
Suppose $\y=\bar{\y}+\z$ where $\bar{\y}=\X\bt_\st$ where $\bt_\st$ lies on the space induced by the top $d$ right singular vectors of $\X$ i.e. $\bt_\st\in\text{range}(\Vb_{1:d})$. Fix $d,R$ and set $r=r(d,R)$ as in Definition \ref{def cov}. Pick iteration count $T=\frac{T_0}{\eta\la_d}$. Set incoherence $\mu=\mu(\Vb_{1:r})$ and the noise projection on top $r$ singular vectors $z_+=\tn{\La_{1:r}^{-1/2}\z'_{1:r}}\leq \tn{\z'_{1:r}}/\sqrt{\la_r}$. Whenever 
\[
\Gamma\geq 2\mu(\e^{-T_0}\tn{\bt_\st}+z_+),
\]
we have that 
\[
|\conf{\bt_\st,\bt_T}|\leq \frac{4T_0^2\tn{\z'_{r+1:p}}^2}{\Gamma^2R\la_d}.
\]%zero-mean 
Now, suppose $\z$ is a random vector with subgaussian norm bounded above by $\sigma$. Set $\mu'=\|\Vb_{1:r}\La_{1:r,1:r}^{-1/2}\|_{2,\infty}\leq \la_r^{-1/2}\|\Vb_{1:r}\|_{2,\infty}$. There exists a constant $C>0$ such that if
\begin{align}
\Gamma\geq C\sigma\sqrt{\log p} (\frac{T_0}{\sqrt{R\la_d}}+\mu')+2\mu \e^{-T_0}\tn{\bt_\st}>2\tn{\bt_T-\bt_\st}.\label{ineq stronger gamma}
\end{align}
then with probability $1-p^{-100}$, we have that $|\conf{\bt_\st,\bt_T}|=0$.
\end{theorem}
\begin{proof} Set the residual at iteration $\tau$ to be $\rb_\tau=\Ub^T(\y-\X\bt_\tau)=\y'-\X'\bt_\tau$ and the initial residual $\rb_0=\y'$. Observe that the residual iteration obeys the power iteration and is dictated by the eigenspectrum
\begin{align}
\rb_\tau&=\Ub^T(\Iden-\eta\X\X^T)^\tau \y=\Ub^T\Ub(\Iden-\eta\X'\X'^T)^\tau\Ub^T \y\\
&(\Iden-\eta\X'\X'^T)^\tau \y'=\sum_{i=1}^n (1-\eta\la_i)^\tau y'_i.
\end{align}
The gradient is given by $\nabla \Lc(\bt_\tau)=\frac{\pa \tn{\y-\X\bt_\tau}^2}{2\pa \bt_\tau}=-\X'^T\rb_\tau$ so that
\begin{align}
\bt_\tau&=\sum_{\tau=0}^{T-1}\eta\nabla \Lc(\bt_\tau)=\eta\sum_{\tau=0}^{T-1} \X'^T\rb_\tau\\
&=\eta\sum_{i=1}^n \sum_{\tau=0}^{T-1} \sqrt{\la_i}(1-\eta\la_i)^\tau y'_i\vb_i=\sum_{i=1}^n (1-(1-\eta\la_i)^{T})\frac{y'_i}{\sqrt{\la_i}} \vb_i,
\end{align}
where we used the fact that $\sum_{\tau=0}^{T-1}\alpha^\tau=\frac{1-\alpha^T}{1-\alpha}$. Now recall that $\y$ can be decomposed as $\y=\bar{\y}+\z$. Recalling $\bar{\y}'=\Ub^T\bar{\y}$ and $\z'=\Ub^T\z$ and using linearity, we find% where $\y=\X\bt+\z$ and similarly represent $\bar{\y}=$ and $\z=$. From linearity, we have that
\[
\bt_\tau=\sum_{i=1}^d (1-(1-\eta\la_i)^{T})\frac{\bar{y}'_i}{\sqrt{\la_i}} \vb_i+\sum_{i=1}^n (1-(1-\eta\la_i)^{T})\frac{z'_i}{\sqrt{\la_i}} \vb_i
\]
where we used the fact that $\bar{\y}$ is in the range of top $d$ eigenvectors. Next observe that the ground-truth parameter has the eigen-representation $\bt_\star=\sum_{i=1}^d \frac{\bar{y}'_i}{\sqrt{\la_i}} \vb_i$ so that the difference satisfies
\[
\bt_T-\bt_\st=-\sum_{i=1}^d (1-\eta\la_i)^{T}\frac{\bar{y}'_i}{\sqrt{\la_i}} \vb_i+\sum_{i=1}^n (1-(1-\eta\la_i)^{T})\frac{z'_i}{\sqrt{\la_i}} \vb_i.
\]
To proceed, we denote $\ab^\dg$ to be the vector with entries $a^\dg_i=\frac{a'_i}{\sqrt{\la_i}}$. % and $\ab^\S$ denotes the vector with entries $a^\S_i=\sqrt{\la_i}a'_i$. 
Define the diagonal matrices $\bar{\Db}=-\text{diag}(\{(1-\eta\la_i)^{T}\}_{i=1}^d)\in\R^{d\times d},~\Db_+=\text{diag}(\{1-(1-\eta\la_i)^{T}\}_{i=1}^r)\in\R^{r\times r},~\Db_-=\text{diag}(\{\frac{1-(1-\eta\la_i)^{T}}{\sqrt{\la_i}}\}_{i=r+1}^p)\in\R^{p-r\times p-r}$. We can now write%Applying triangle inequality, we find
\begin{align}
&\bt_\tau-\bt_\star=\underbrace{\Vb_{1:d}\bar{\Db}\bar{\y}^\dg_{1:d}}_{\bar{\y}^\S}+\underbrace{\Vb_{1:r}\Db_+\z^\dg_{1:r}}_{\z^\S_+}+\underbrace{\Vb_{r+1:p}\Db_-\z'_{r+1:p}}_{\z^\S_-}.
%&\tin{\bt_\tau-\bt_\star}\leq \tin{\Vb_{1:d}\bar{\Db}\bar{\y}^\dg_{1:d}}+\tin{\Vb_{1:r}\Db_+\z^\dg_{1:r}}+\tin{\Vb_{r+1:p}\Db_-\z_{r+1:p}}.
\end{align}
To simplify the results, we next apply the following standard bound
\[
1-\frac{T_0\la_i}{\la_d}= 1-T\eta \la_i\leq (1-\eta\la_i)^T\leq \e^{-T\eta \la_i}= \e^{-T_0 \frac{\la_i}{\la_d}}.
\]
For $i\leq d$, this guarantees that $(1-\eta\la_i)^{T}\leq \e^{-T_0}$. In contrast, for $i\geq r$, we find that $1-\frac{T_0\la_i}{\la_d}\geq 1-\frac{T_0}{R}$. Consequently, for individual terms, we obtain the following after setting $\mu=\mu(\Vb_{1:r})$.
\begin{itemize}
\item Observe that $\bar{\y}^\dg=\tn{\bt_\st}$. Hence 
\[
\tin{\bar{\y}^\S}\leq \mu(\Vb_{1:d})\|\bar{\Db}\|\|\Vb_{1:d}\|\tn{\bar{\y}^\dg_{1:d}}\leq \e^{-T_0}\mu(\Vb_{1:d})\tn{\bt_\st}\leq \e^{-T_0}\mu\tn{\bt_\st}.
\]
\item Similarly, using $\|\Db_+\|\leq 1$, we find
\[
\tin{\z^\S_+}\leq \mu(\Vb_{1:r})\tn{\z^\dg_{1:r}}=\mu \tn{\z^\dg_{1:r}}.
\]
\item Finally using $\la_i\leq \la_d/R$ for $i\geq r+1$, we find $\|\Db_{-}\|\leq \sup_{p\geq i\geq r+1}\frac{1-(1-\eta\la_i)^{T}}{\sqrt{\la_i}}\leq \frac{T_0\sqrt{\la_i}}{\la_d}\leq \frac{T_0}{\sqrt{R\la_d}}$. This yields
\[
\tn{\z^\S_-}\leq \frac{T_0}{\sqrt{R\la_d}}\tn{\z'_{r+1:p}}.
\]
Next, define the multiplication incoherence as $\mu(\M,\vb)=\frac{\tin{\M\vb}}{\|\M\|\tn{\vb}}$ and denote
\[
\mu_{z,-}=\mu(\Vb_{r+1:p},\Db_-\z'_{r+1:p}).
\]
With this, we obtain
\[
\tin{\z^\S_-}\leq\mu_{z,-} \tn{\Db_-\z'_{r+1:p}}\leq \frac{T_0}{\sqrt{R\la_d}}\mu_{z,-}\tn{\z'_{r+1:p}}.
\]
\end{itemize}
\noindent{\bf{Deterministic analysis:}} To proceed, we are in a position to apply Lemma \ref{lem robust} with $\bb=\bar{\y}^\S+\z^\S_+$ and $\ab=\z^\S_-$. Specifically, if the feature importance threshold $\Gamma$ satisfies
\[
\Gamma\geq 2\mu(\e^{-T_0}\tn{\bt_\st}+\tn{\z^\dg_{1:r}})\geq 2\tin{\bb},
\]
we can bound the confusion set between $\bt_\st$ and $\bt_T$ by
\[
\conf{\bt_T,\bt_\st}\leq \frac{4T_0^2\tn{\z'_{r+1:p}}^2}{\Gamma^2R\la_d}.
\]

\noindent{\bf{Randomized analysis:}} Next, we would like to obtain a guarantee when $\z$ has bounded subgaussian norm $\tsub{\z}\leq \sigma$. In this case, first note that subgaussian norm of $\z^\S_-$ obeys
\[
\tsub{\z^\S_-}\leq c\|\Vb_{r+1:p}\| \|\Db_-\| \tsub{\z'}\leq c\frac{T_0}{\sqrt{R\la_d}}\sigma.
\]
Similarly, rewrite $\z^\S_+=\Vb_{1:r}\La_{1:r,1:r}^{-1/2}\z'_{1:r}$. Hence $\tsub{\z^\S_+}\leq c\sigma\mu'$.
Hence, using subgaussian tail and union bounding, there exists a constant $C>0$ such that with probability $1-p^{-100}$, 
\begin{itemize}
\item $\tin{\z^\S_-}\leq \frac{CT_0\sqrt{\log p}}{\sqrt{R\la_d}}\sigma$.
\item $\tin{\z'_{1:r}}\leq C\sigma\sqrt{\log p}\mu'$.% so that $\tin{\z^\S_+}\leq C\mu\sigma\sqrt{\sum_{i=1}^r\la_i^{-1}\log p}\leq C\mu\sigma\sqrt{\frac{r}{\la_r}\log p}$.
\end{itemize}
Consequently, with the same probability, we find that
\[
\tin{\bt_T-\bt_\st}\leq \frac{\Gamma_0}{2}=C\sigma\sqrt{\log p} (\frac{T_0}{\sqrt{R\la_d}}+\mu')+\mu \e^{-T_0}\tn{\bt_\st}.
\]
Hence, applying Lemma \ref{lem robust} with $\ab=0$ and $\bb=\bt_T-\bt_\st$, whenever $\Gamma\geq \Gamma_0$, we conclude with the desired statement $|\conf{\bt_T,\bt_\st}|=0$.
\end{proof}

%\begin{lemma}[Shrinkage lemma] Let $\bt_\st$ be an $s$-sparse vector and suppose $\bt'=\bt_\st+\ab+\bb$ where $\tin{\bb}\leq \gamma$. Then for $\la\geq \gamma$, $\hat{\bt}=\prox{\la}(\bt')$ obeys $\tn{\hat{\bt}-\bt_\st}\leq \tn{\ab}+2\sqrt{s}\la$.
%\end{lemma}
%\begin{proof} Let $S$ be the support of $\bt_\st$. For $i\in S$, we have that
%\[
%|\shr{\la}{\bt_\st[i]+\ab[i]+\bb[i]}-\bt_\st[i]|\leq |\ab[i]|+|\bb[i]|+\la\leq  |\ab[i]|+2\la.
%\]
%For $i\in S^c$, we have
%\[
%|\shr{\la}{\ab[i]+\bb[i]}|\leq \max(0,|\ab[i]|+|\bb[i]|-\la)\leq  |\ab[i]|.
%\]
%Combining these, we find the desired result.
%\end{proof}
