# Supplementary material for: Exploring Weight Importance and Hessian Bias in Model Pruning
Source: arXiv:2006.10903 source file (2020-06-19)
Supplement: Supplementary file 2 [file appendix_experiments.tex]

\section{Additional experiments}

\subsection{Neural network}

\begin{figure*}[t!]
	\begin{subfigure}{2.2in}
		\begin{tikzpicture}
		\node at (0,0) {\includegraphics[scale=0.38]{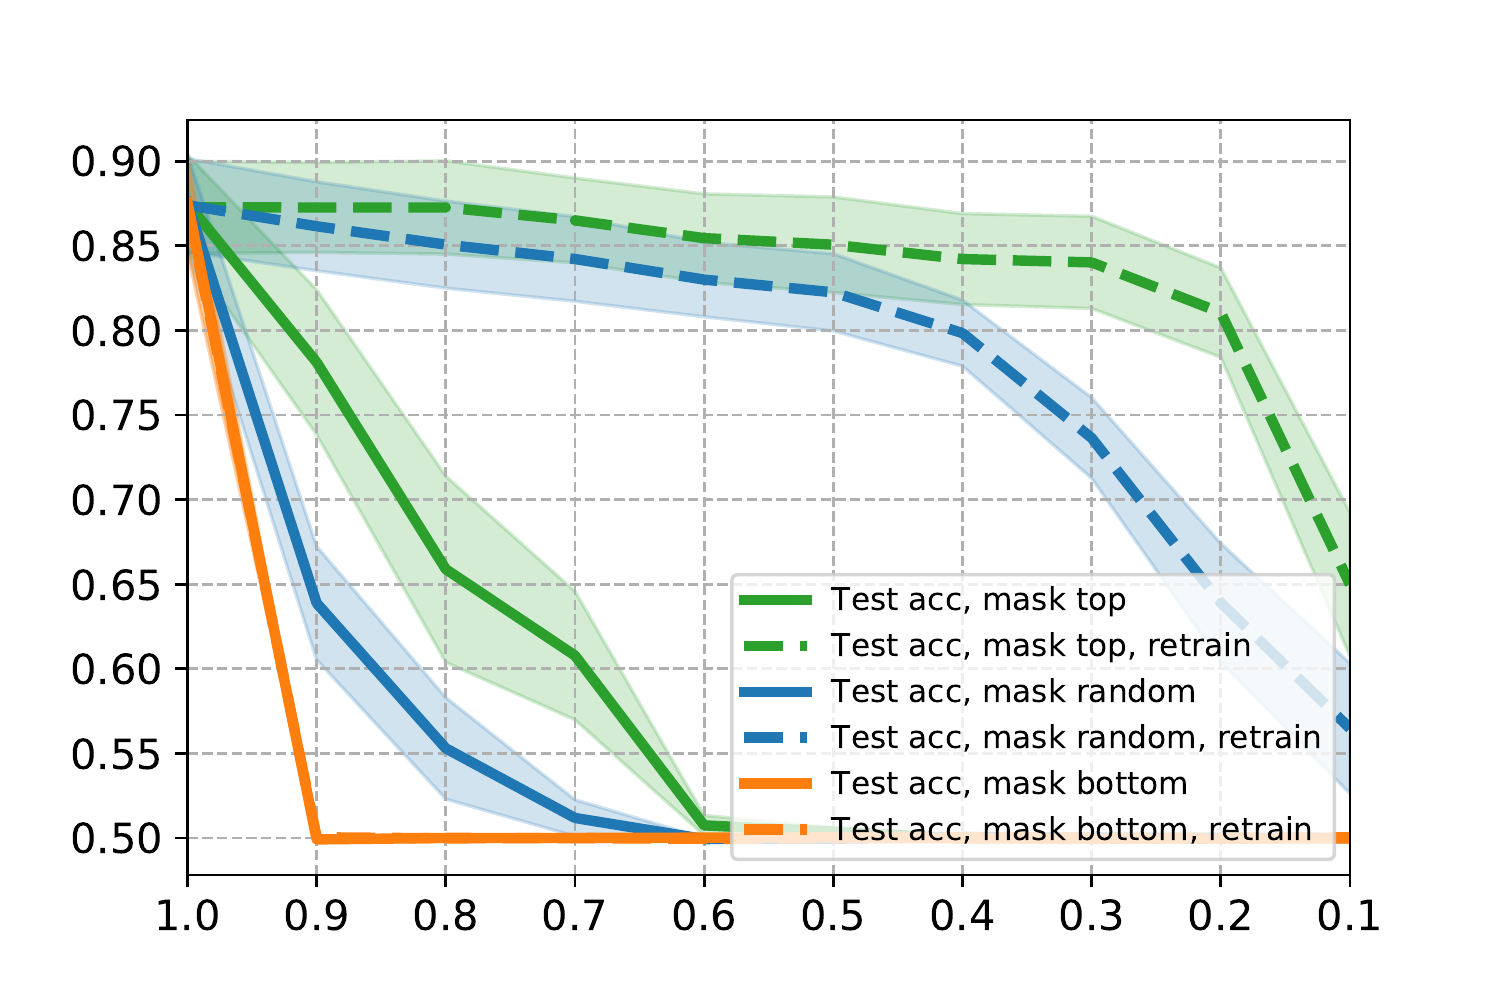}};
		\node at (-3,0) [rotate=90,scale=.8]{Test accuracy};
		\node at (0,-2.1) [scale=.8]{Fraction of non-zero};
		\end{tikzpicture}\caption{Test accuracy on multiple pruning level. \\ \quad}\label{fig:app_distance_1}
	\end{subfigure}
	\begin{subfigure}{2.2in}
		\begin{tikzpicture}
		\node at (0,0) {\includegraphics[scale=0.38]{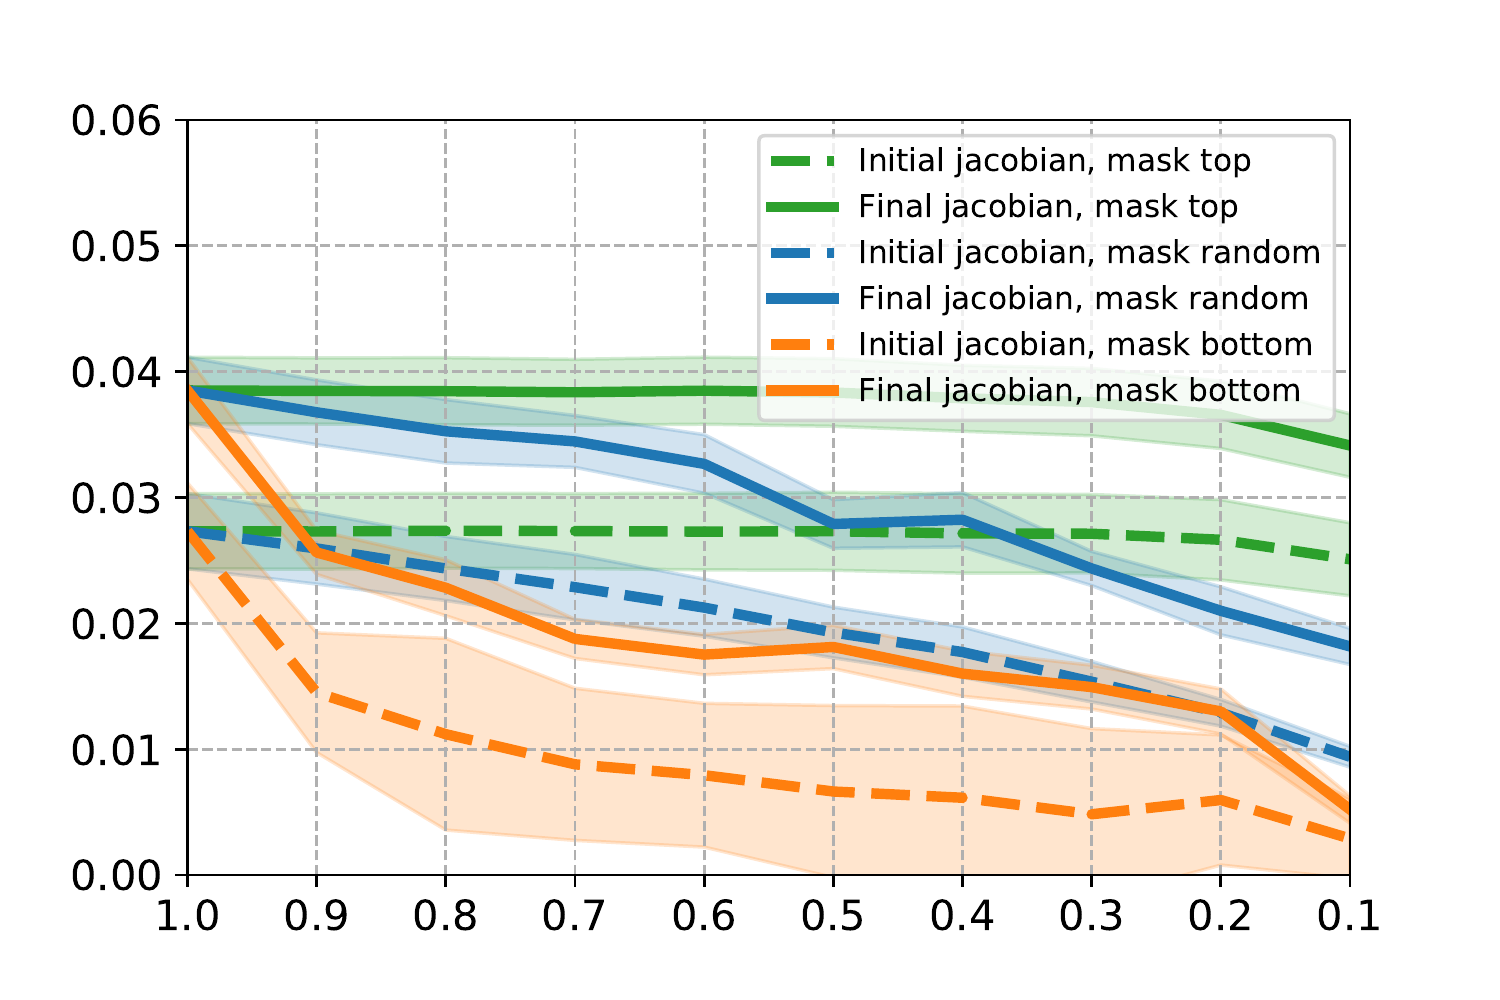}};
		\node at (-3,0) [rotate=90,scale=.8]{Jacobian Correlation};
		\node at (0,-2.1) [scale=.8]{Fraction of non-zero};
		\end{tikzpicture}\caption{Correlation between the weights and the Jacobian matrix for varying level of pruning.}\label{fig:app_distance_2} 
	\end{subfigure}
	\begin{subfigure}{2.2in}
		\begin{tikzpicture}
		\node at (0,0) {\includegraphics[scale=0.38]{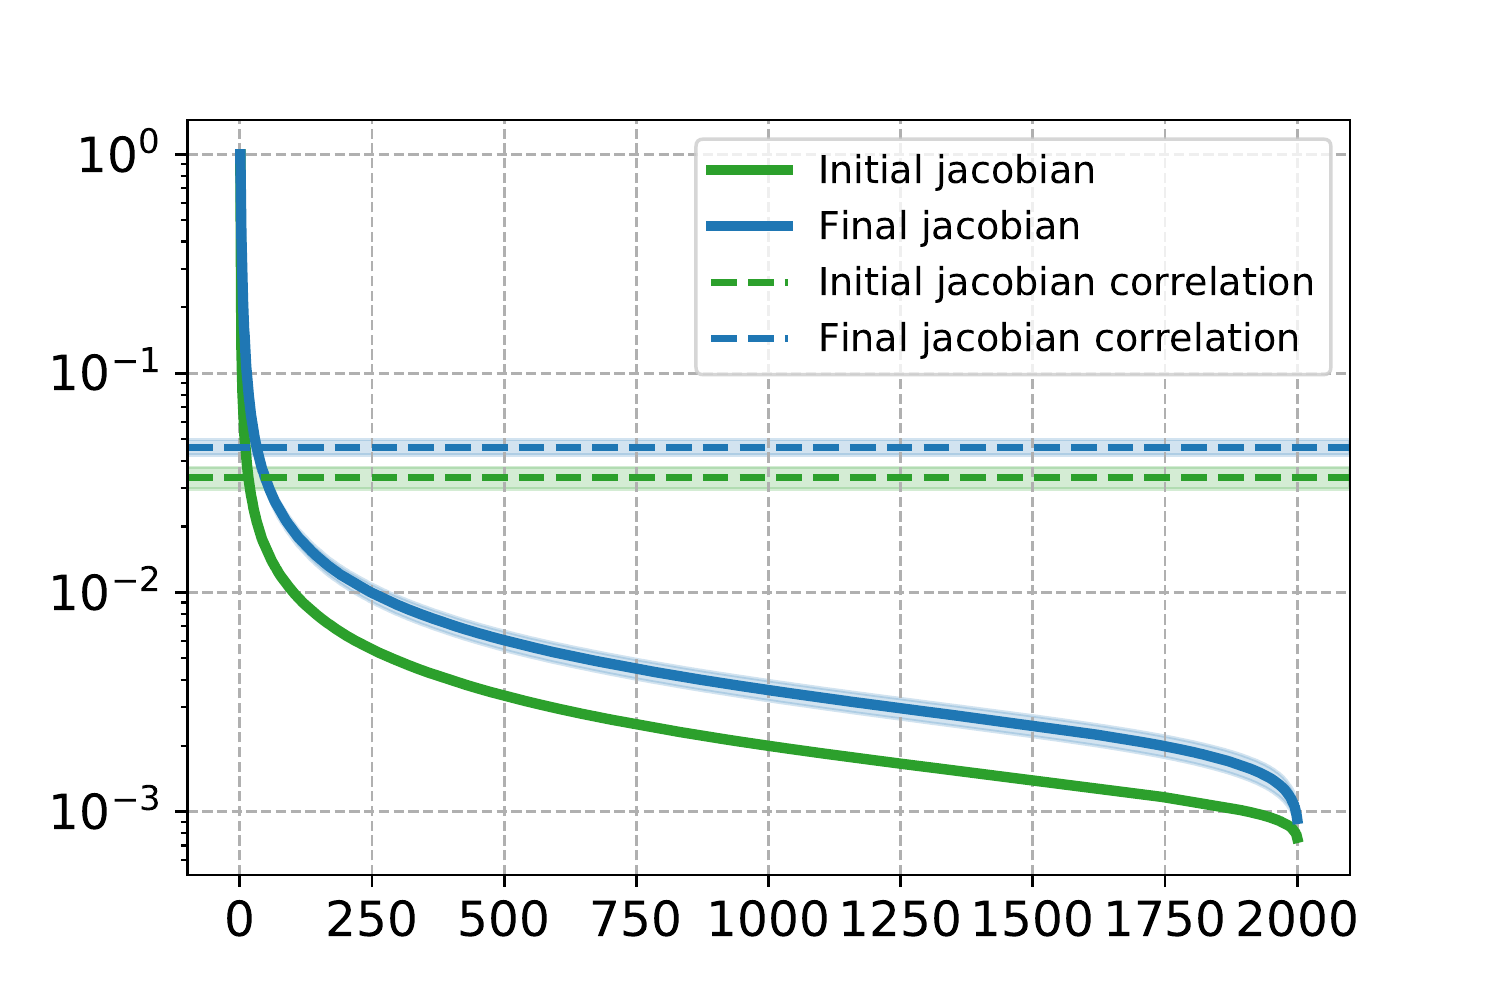}};
		\node at (-3,0) [rotate=90,scale=.8]{Normalized singular value};
		\node at (0,-2.1) [scale=.8]{Index of singular value};
		\end{tikzpicture}\caption{Jacobian spectrum and correlation of the distance vector $\bar{\bt}_{final}$ with the Jacobian.}\label{fig:app_distance_3} 
	\end{subfigure}
	\caption{Distance pruning. Fig.~\ref{fig:app_distance_2} and solid line in \ref{fig:app_distance_1} shows the correlation and test accuracy on pruned weight $\bt_{final}^{prune}=m_{distance}^p\odot\bt_{final}$  where $m_{distance}^p=\text{mask}^p(\bt_{final}-\bt_0)$. The dash line in Fig.~\ref{fig:app_distance_1} shows the retrained test accuracy when training from $\bt^{prune}_{0}=m_{distance}^p\odot\bt_{0}$ with mask $m_{distance}^p$ which only update weight on masked entries as $\nabla\Lc_{masked}=m_{distance}^p\odot\nabla\Lc$.}\label{fig:app_distance} \vspace{-0.3cm}
\end{figure*}

\begin{figure*}[t!]
	\begin{subfigure}{2.2in}
		\begin{tikzpicture}
		\node at (0,0) {\includegraphics[scale=0.38]{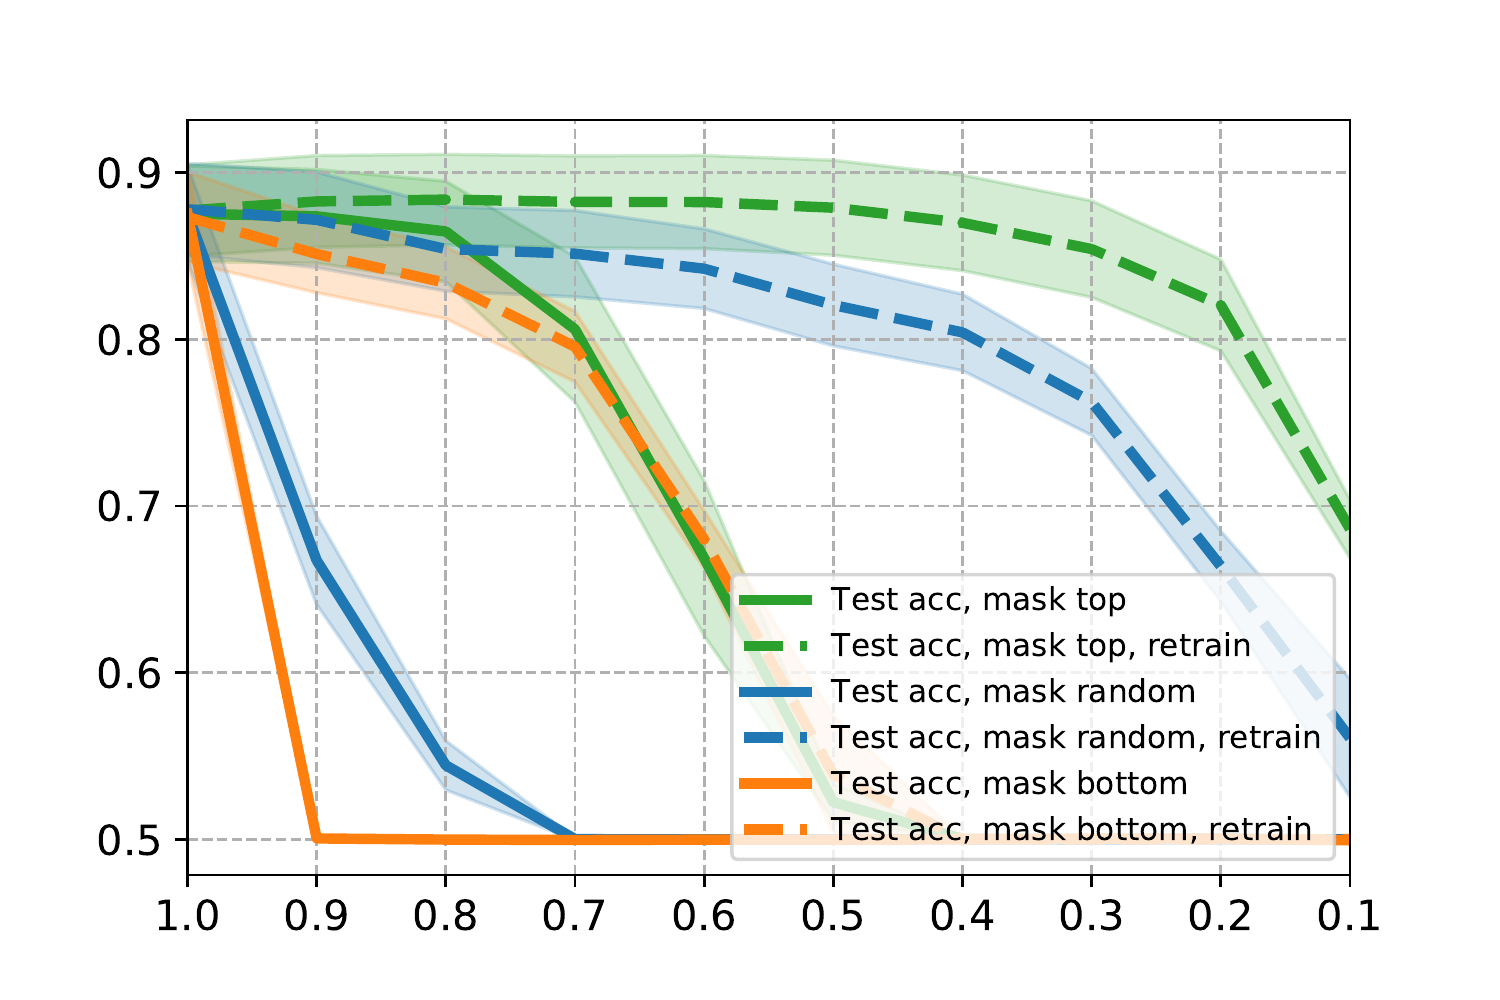}};
		\node at (-3,0) [rotate=90,scale=.8]{Test accuracy};
		\node at (0,-2.1) [scale=.8]{Fraction of non-zero};
		\end{tikzpicture}\caption{Test accuracy on multiple pruning level. \\ \quad}\label{fig:app_weight_1}
	\end{subfigure}
	\begin{subfigure}{2.2in}
		\begin{tikzpicture}
		\node at (0,0) {\includegraphics[scale=0.38]{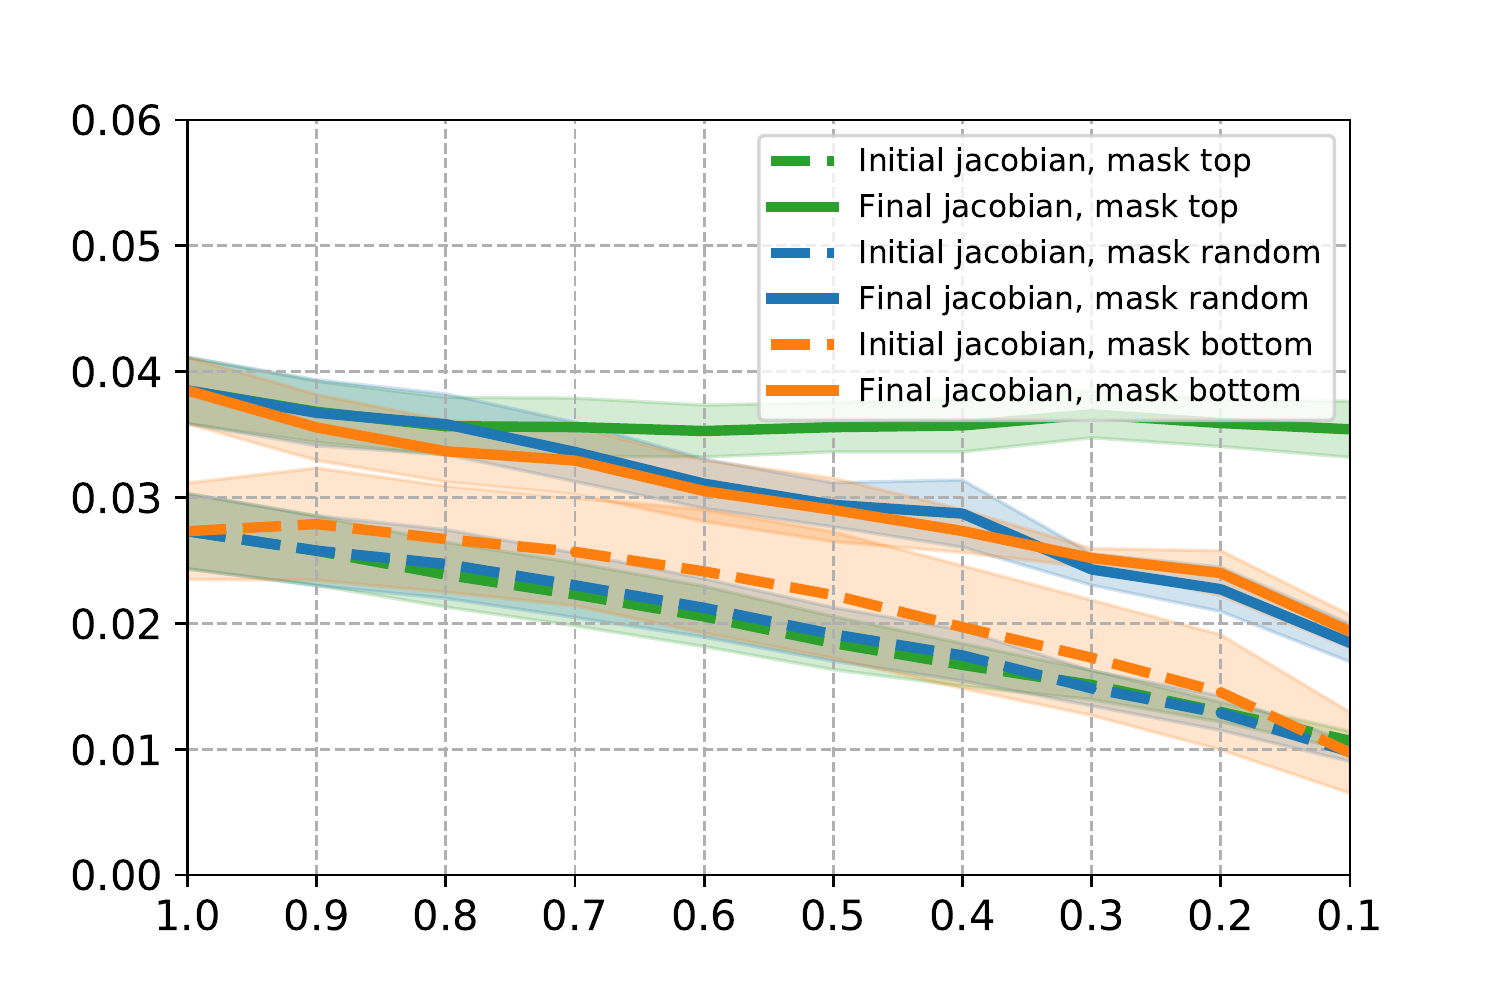}};
		\node at (-3,0) [rotate=90,scale=.8]{Jacobian Correlation};
		\node at (0,-2.1) [scale=.8]{Fraction of non-zero};
		\end{tikzpicture}\caption{Correlation between the weights and the Jacobian matrix for varying level of pruning.}\label{fig:app_weight_2} 
	\end{subfigure}
	\begin{subfigure}{2.2in}
		\begin{tikzpicture}
		\node at (0,0) {\includegraphics[scale=0.38]{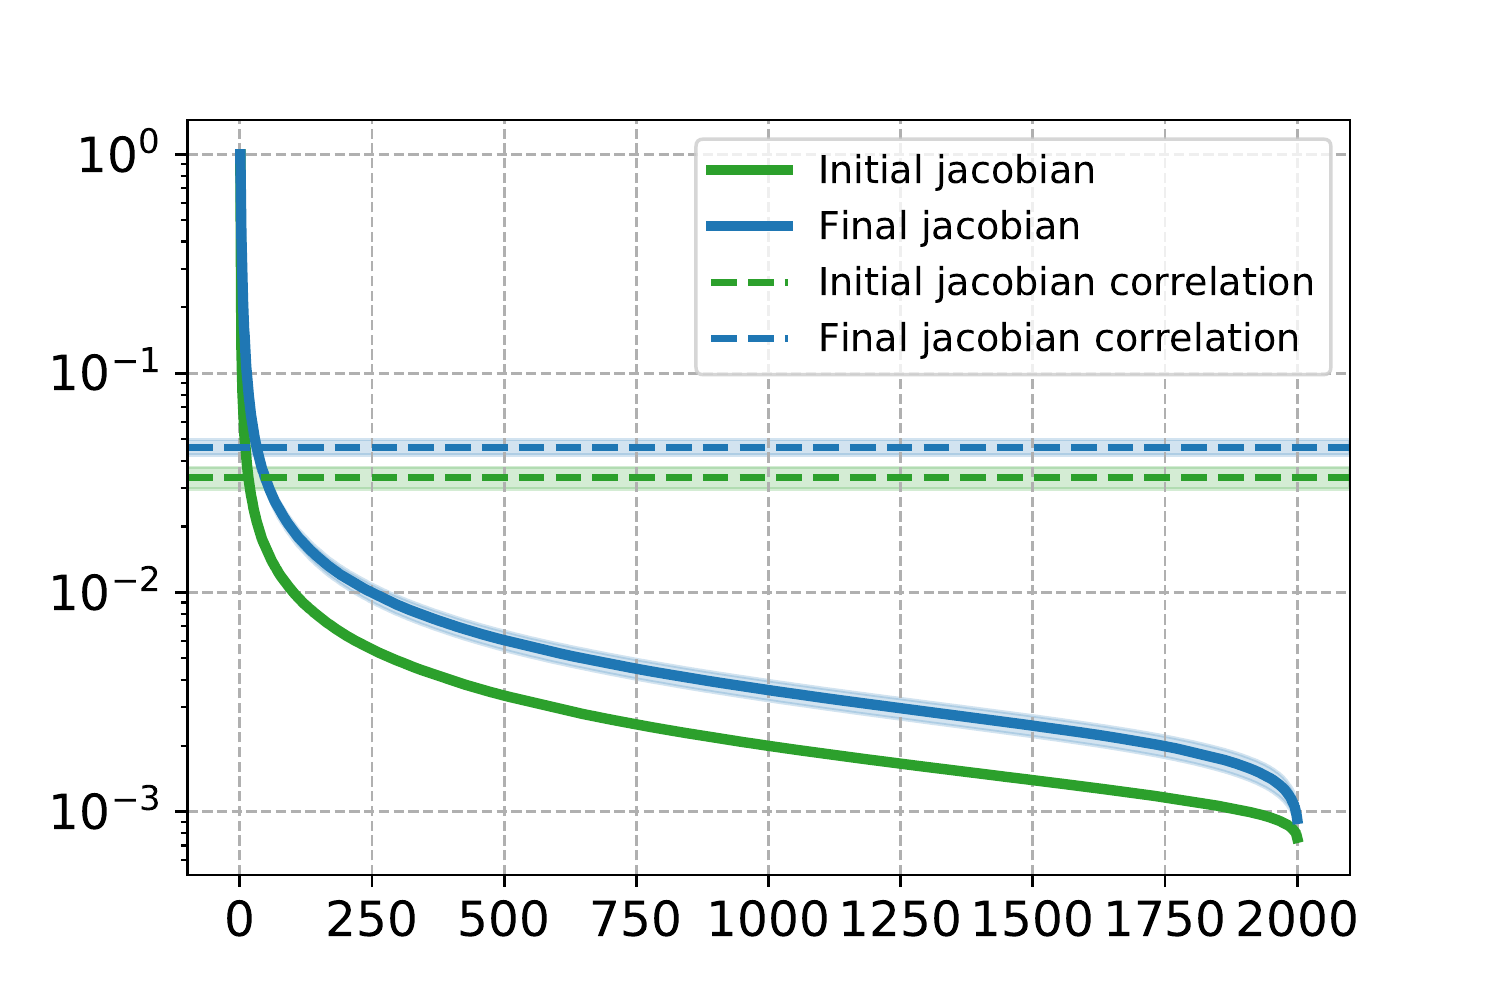}};
		\node at (-3,0) [rotate=90,scale=.8]{Normalized singular value};
		\node at (0,-2.1) [scale=.8]{Index of singular value};
		\end{tikzpicture}\caption{Jacobian spectrum and correlation of the distance vector $\bar{\bt}_{final}$ with the Jacobian.}\label{fig:app_weight_3} 
	\end{subfigure}
	\caption{Weight pruning. Fig.~\ref{fig:app_weight_2} and solid line in \ref{fig:app_weight_1} shows the correlation and test accuracy on pruned weight $\bt_{final}^{prune}=m_{weight}^p\odot\bt_{final}$  where $m_{weight}^p=\text{mask}^p(\bt_{final})$. The dash line in Fig.~\ref{fig:app_weight_1} shows the retrained test accuracy when training from $\bt^{prune}_{0}=m_{weight}^p\odot\bt_{0}$ with mask $m_{weight}^p$ which only update weighton masked entries as $\nabla\Lc_{masked}=m_{weight}^p\odot\nabla\Lc$.}\label{fig:app_weight} \vspace{-0.3cm}
\end{figure*}

\begin{figure*}[t!]
	\begin{subfigure}{2.2in}
		\begin{tikzpicture}
		\node at (0,0) {\includegraphics[scale=0.38]{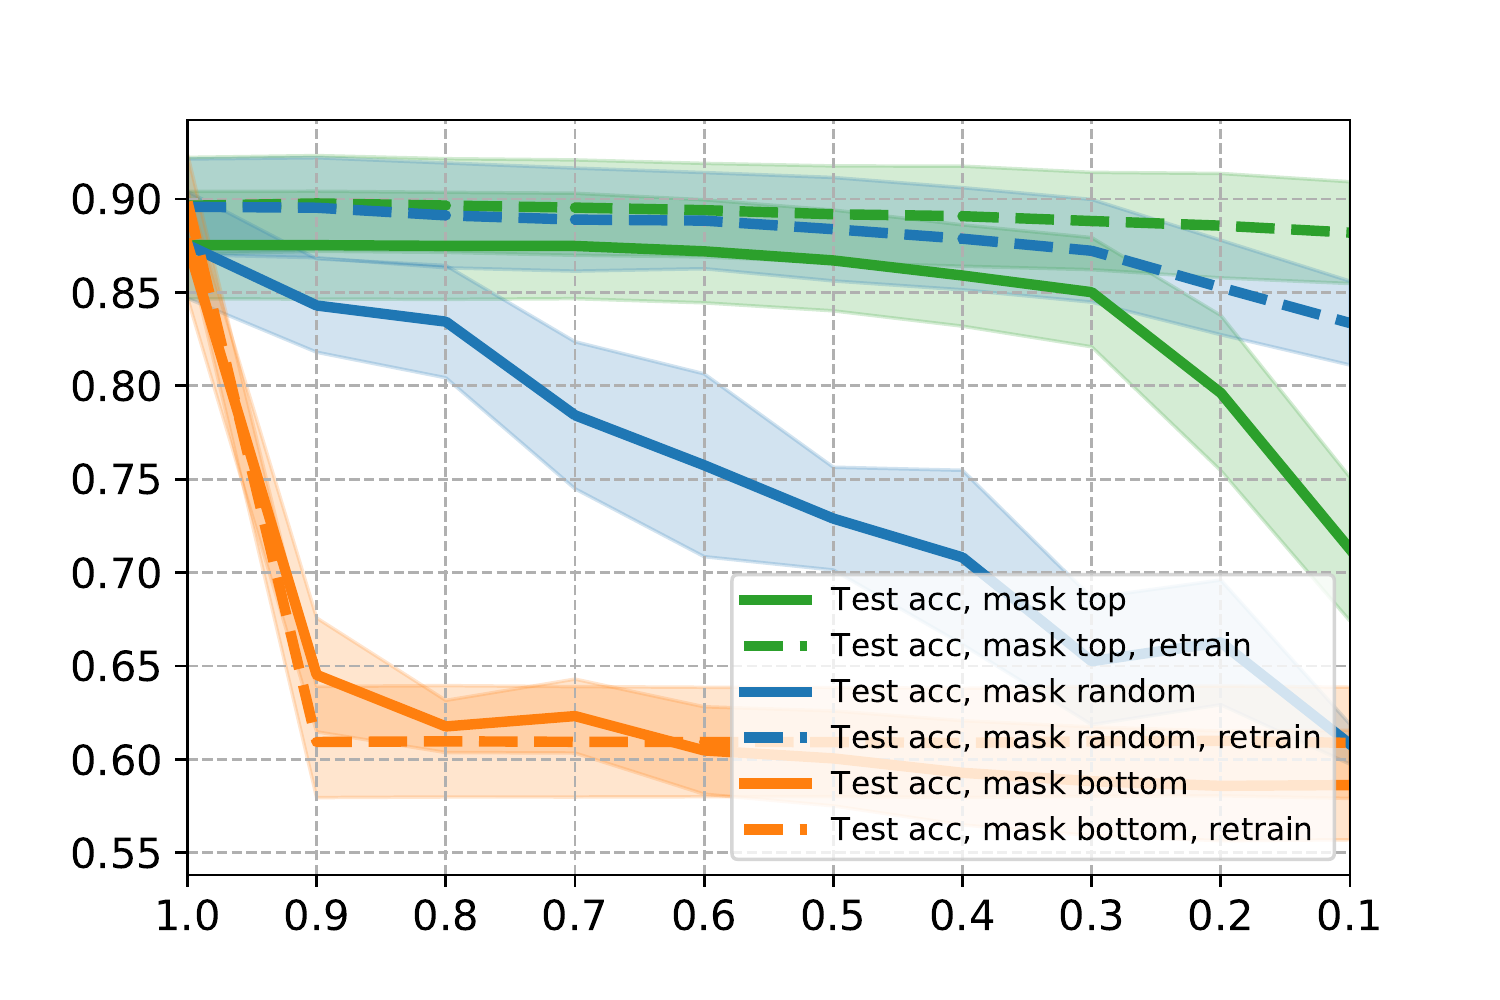}};
		\node at (-3,0) [rotate=90,scale=.8]{Test accuracy};
		\node at (0,-2.1) [scale=.8]{Fraction of non-zero};
		\end{tikzpicture}\caption{Test accuracy on multiple pruning level. \\ \quad}\label{fig:app_theory_1}
	\end{subfigure}
	\begin{subfigure}{2.2in}
		\begin{tikzpicture}
		\node at (0,0) {\includegraphics[scale=0.38]{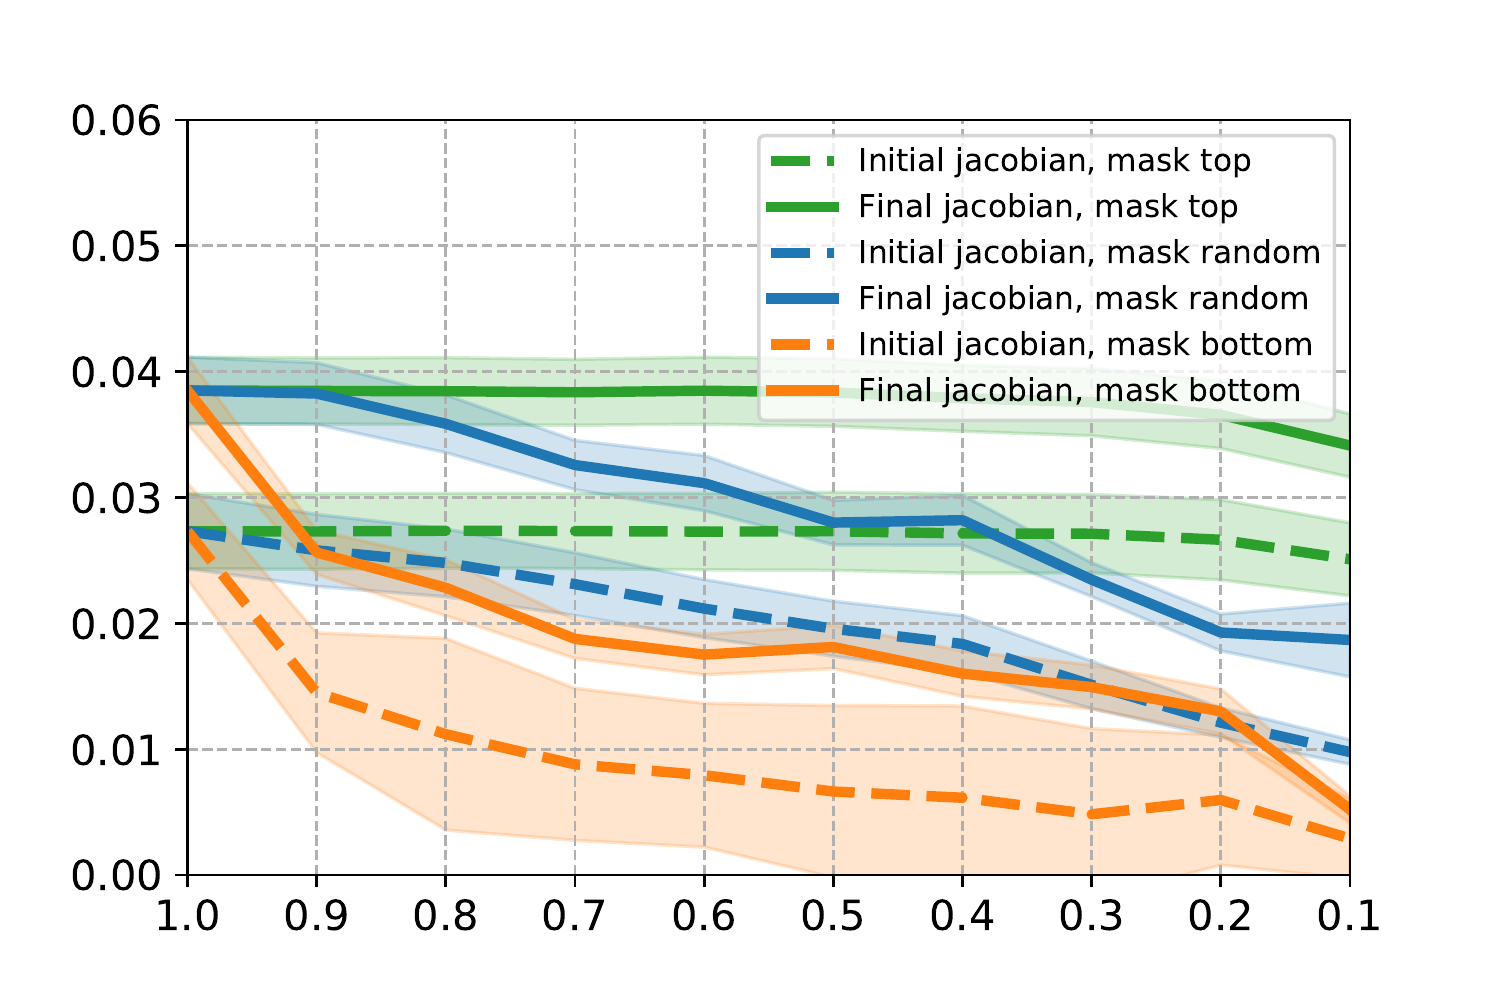}};
		\node at (-3,0) [rotate=90,scale=.8]{Jacobian Correlation};
		\node at (0,-2.1) [scale=.8]{Fraction of non-zero};
		\end{tikzpicture}\caption{Correlation between the weights and the Jacobian matrix for varying level of pruning.}\label{fig:app_theory_2} 
	\end{subfigure}
	\begin{subfigure}{2.2in}
		\begin{tikzpicture}
		\node at (0,0) {\includegraphics[scale=0.38]{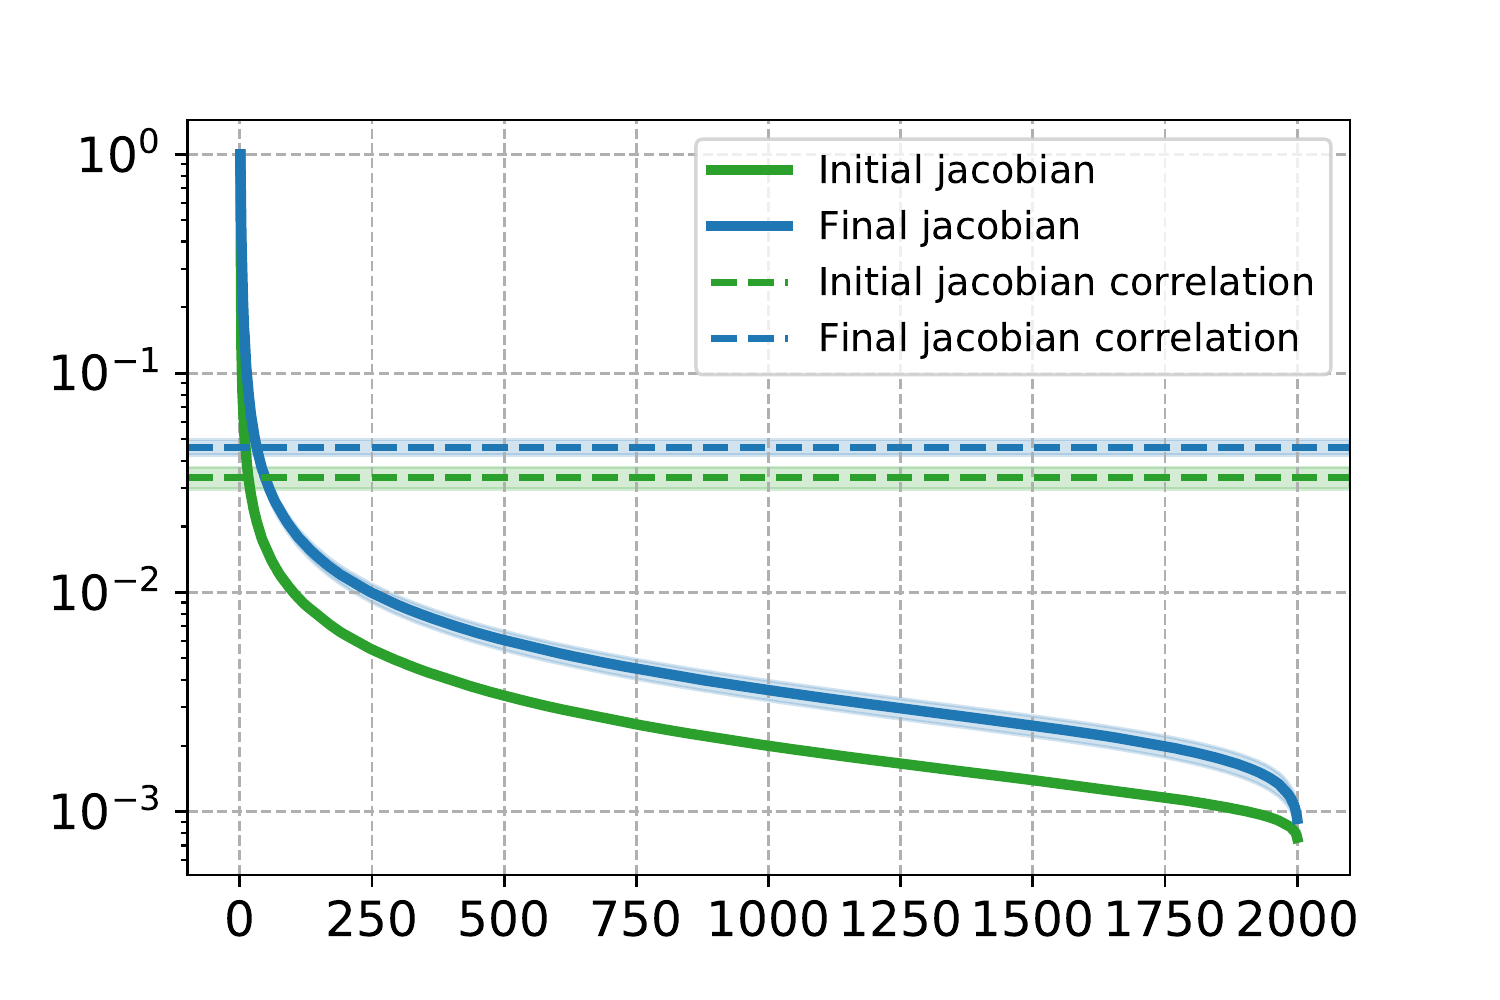}};
		\node at (-3,0) [rotate=90,scale=.8]{Normalized singular value};
		\node at (0,-2.1) [scale=.8]{Index of singular value};
		\end{tikzpicture}\caption{Jacobian spectrum and correlation of the distance vector $\bar{\bt}_{final}$ with the Jacobian.}\label{fig:app_theory_3} 
	\end{subfigure}
	\caption{Distance pruning \& set initial. Fig.~\ref{fig:app_theory_2} and solid line in \ref{fig:app_theory_1} shows the correlation and test accuracy on pruned weight $\bt_{final}^{prune}=m_{distance}^p\odot\bt_{final}+(\mathds{1}-m_{distance}^p)\odot\bt_{0}$  where $m_{distance}^p=\text{mask}^p(\bt_{final}-\bt_0)$. The dash line in Fig.~\ref{fig:app_theory_1} shows the retrained test accuracy when training from $\bt^{prune}_{0}=\bt_{0}$ with mask $m_{distance}^p$ which only update weight on masked entries as $\nabla\Lc_{masked}=m_{distance}^p\odot\nabla\Lc$}. \label{fig:app_theory} \vspace{-0.3cm}
\end{figure*}

\begin{figure*}[t!]
	\begin{subfigure}{2.2in}
		\begin{tikzpicture}
		\node at (0,0) {\includegraphics[scale=0.38]{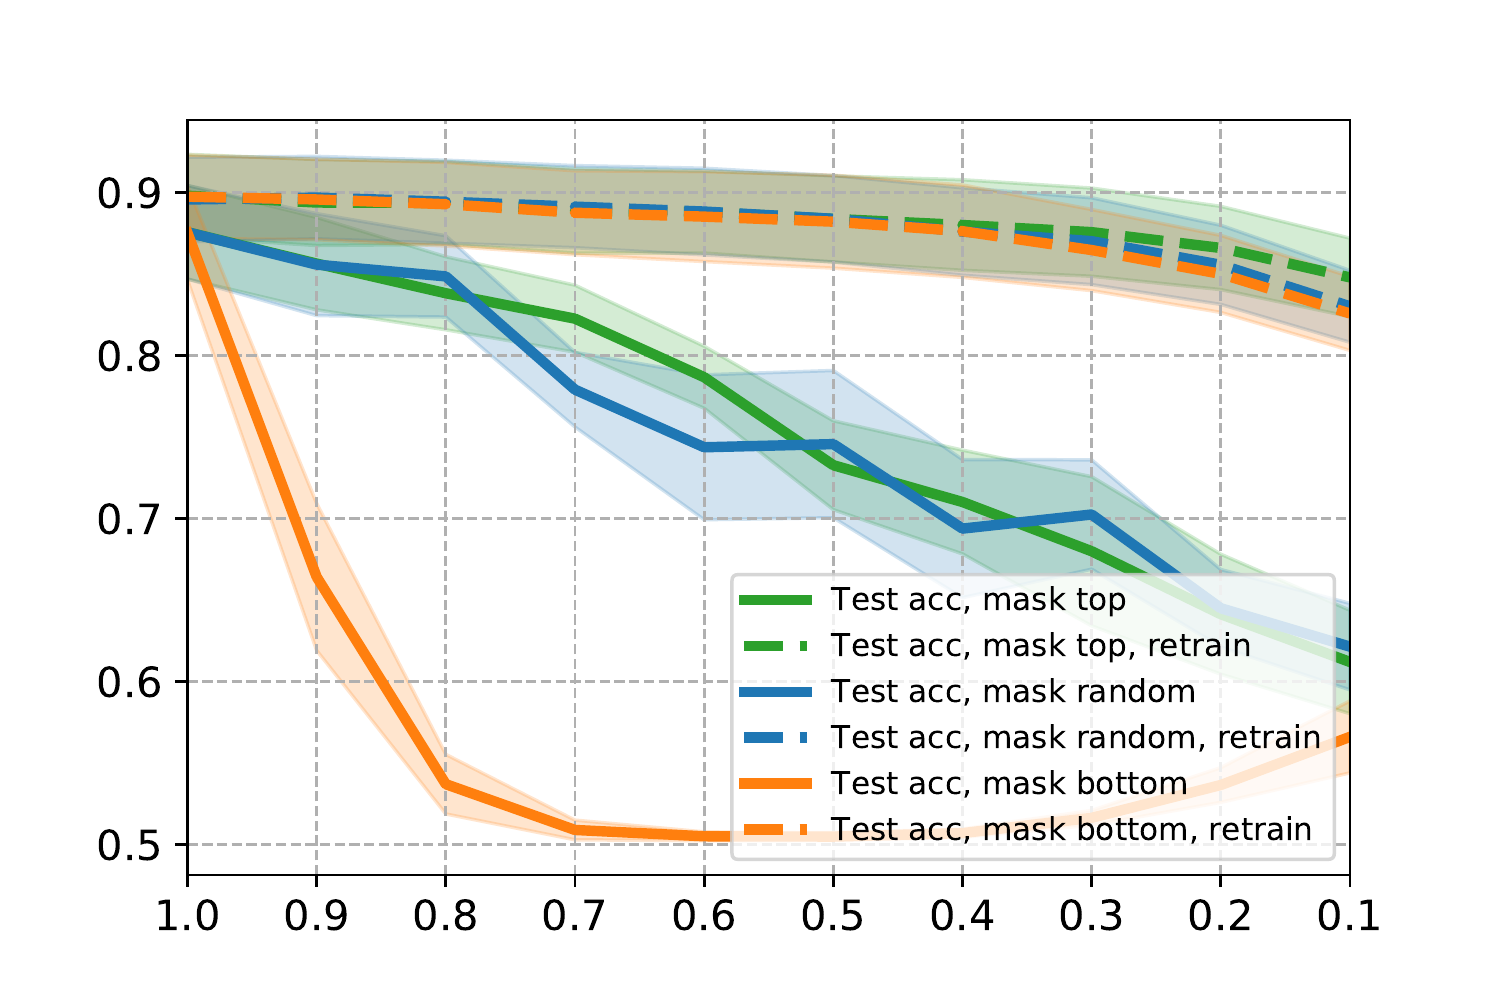}};
		\node at (-3,0) [rotate=90,scale=.8]{Test accuracy};
		\node at (0,-2.1) [scale=.8]{Fraction of non-zero};
		\end{tikzpicture}\caption{Test accuracy on multiple pruning level. \\ \quad}\label{fig:app_weight_init_1}
	\end{subfigure}
	\begin{subfigure}{2.2in}
		\begin{tikzpicture}
		\node at (0,0) {\includegraphics[scale=0.38]{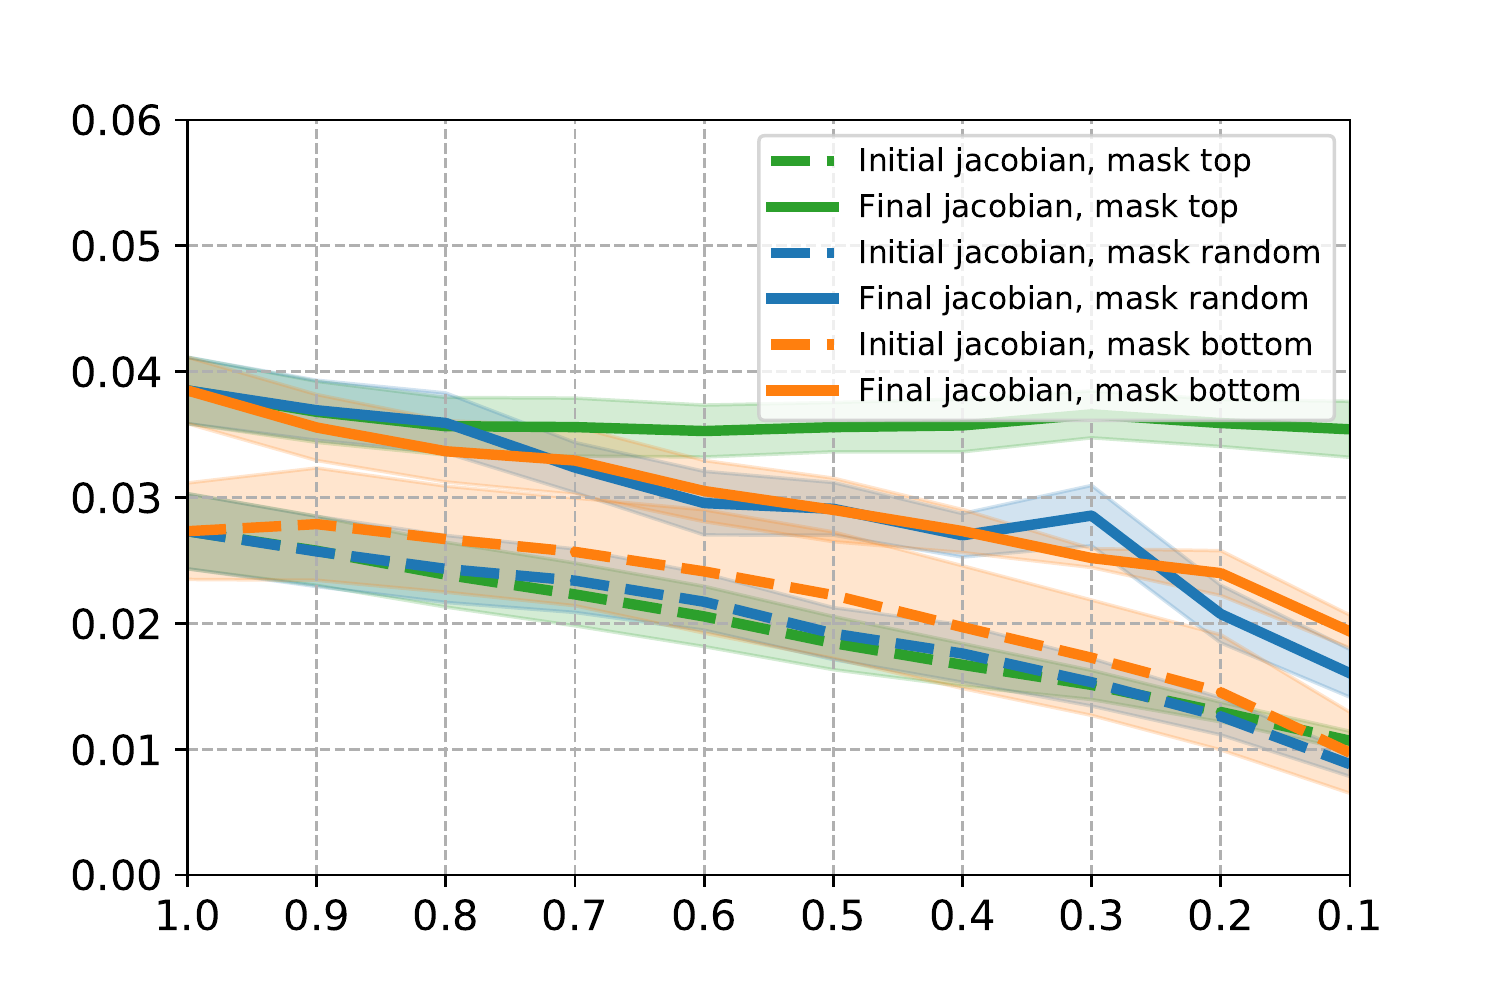}};
		\node at (-3,0) [rotate=90,scale=.8]{Jacobian Correlation};
		\node at (0,-2.1) [scale=.8]{Fraction of non-zero};
		\end{tikzpicture}\caption{Correlation between the weights and the Jacobian matrix for varying level of pruning.}\label{fig:app_weight_init_2} 
	\end{subfigure}
	\begin{subfigure}{2.2in}
		\begin{tikzpicture}
		\node at (0,0) {\includegraphics[scale=0.38]{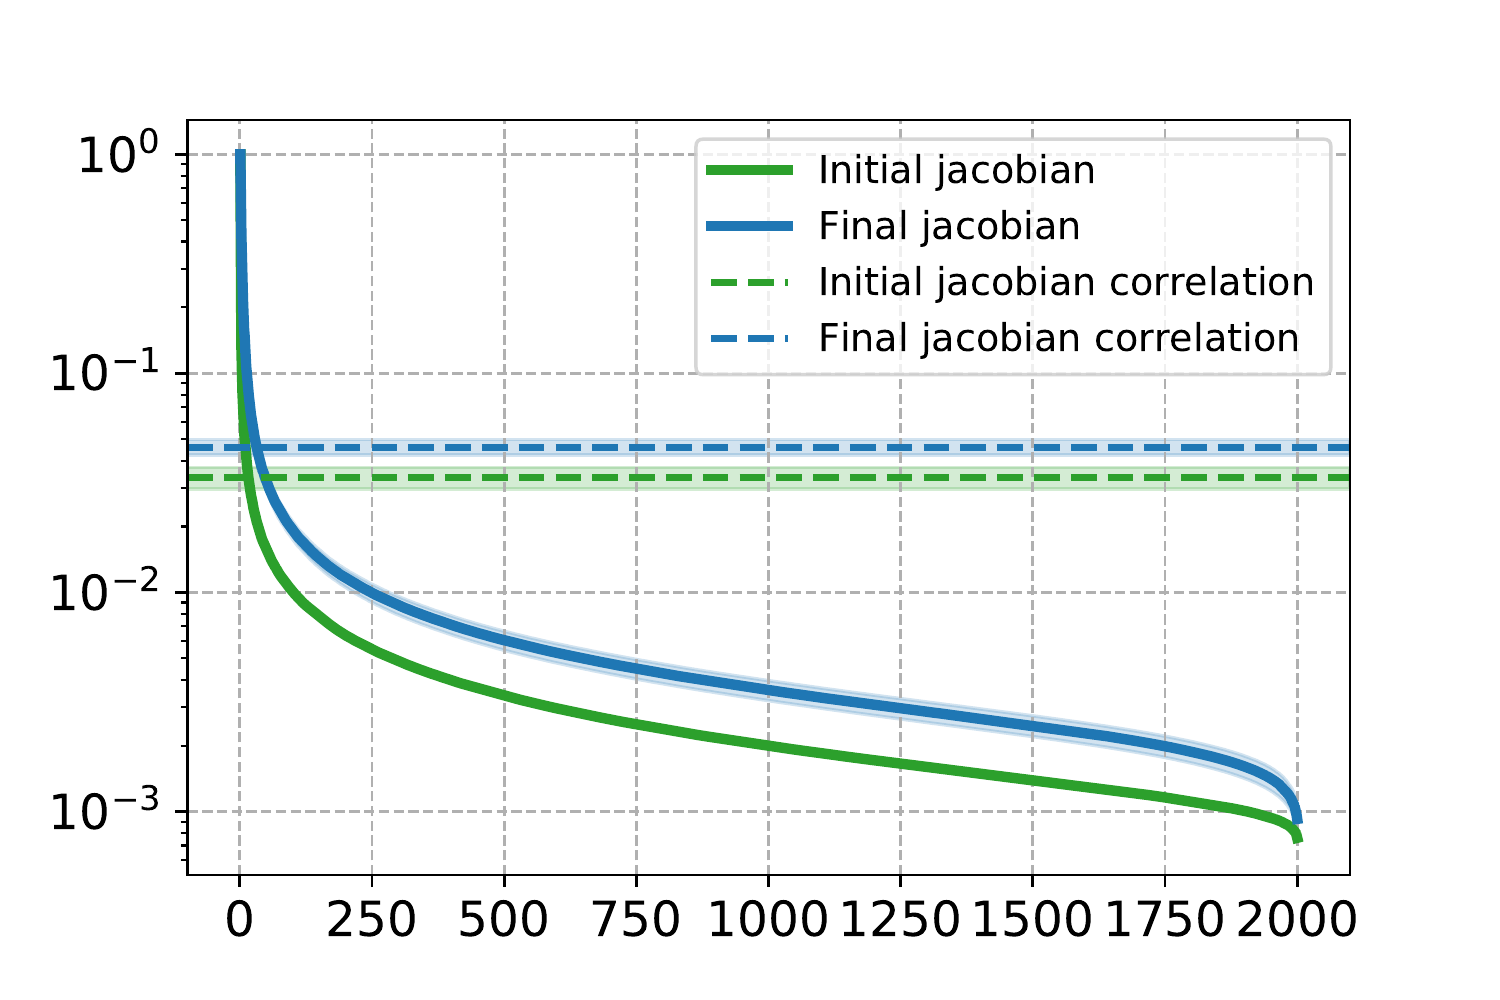}};
		\node at (-3,0) [rotate=90,scale=.8]{Normalized singular value};
		\node at (0,-2.1) [scale=.8]{Index of singular value};
		\end{tikzpicture}\caption{Jacobian spectrum and correlation of the distance vector $\bar{\bt}_{final}$ with the Jacobian.}\label{fig:app_weight_init_3} 
	\end{subfigure}
	\caption{Weight pruning \& set initial. Fig.~\ref{fig:app_weight_init_2} and solid line in \ref{fig:app_weight_init_1} shows the correlation and test accuracy on pruned weight $\bt_{final}^{prune}=m_{weight}^p\odot\bt_{final}+(\mathds{1}-m_{weight}^p)\odot\bt_{0}$  where $m_{weight}^p=\text{mask}^p(\bt_{final})$. The dash line in Fig.~\ref{fig:app_weight_init_1} shows the retrained test accuracy when training from $\bt^{prune}_{0}=m_{weight}^p\odot\bt_{0}$ with mask $m_{weight}^p$ which only update weight on masked entries as $\nabla\Lc_{masked}=m_{weight}^p\odot\nabla\Lc$ }\label{fig:app_weight_init} \vspace{-0.3cm}
\end{figure*}

In this section, we compare among four pruning methods and show the results in Fig.~\ref{fig:app_distance},~\ref{fig:app_weight},~\ref{fig:app_theory} and ~\ref{fig:app_weight_init}. Let us use \textit{distance pruning} $m_{distance}^p=\text{mask}^p(\bt_{final}-\bt_0)$ to denote the pruning method that masks weight by its moving distance while training. And use \textit{weight pruning} to denote the pruning method that only considers the top entries of final weight ($m_{weight}^p=\text{mask}^p(\bt_{final})$). In both methods, we compute the pruned final weight by $\bt_{final}^{prune}=m^p\odot\bt_{final}$ and set other entries to 0. However, the third pruning method uses $\bt_{final}^{prune}=m_{distance}^p\odot\bt_{final}+(\mathds{1}-m_{distance}^p)\odot\bt_{0}$ which firstly masks final weight by distance pruning $m_{distance}^p$ and then set other entries to initial weight. We call the third method \textit{distance pruning \& set initial} which is consistent to Thm.~\ref{lem small grad}. And the fourth method which we called \textit{weight pruning \& set initial} firstly masks weight according to magnitude of final weight and then set other entries to initial weight which is $\bt_{final}^{prune}=m_{weight}^p\odot\bt_{final}+(\mathds{1}-m_{weight}^p)\odot\bt_{0}$.

Fig.~\ref{fig:app_gradient_fraction_distance} and ~\ref{fig:app_gradient_fraction_weight} shows the evolution of energy and fraction for top and bottom 10\% masking on CIFAR-10 dataset. The figures show that top entries consistently maintain higher energy and fraction both on gradient of loss and magnitude of weights than bottom entries.

\begin{figure*}[t!]
	\begin{subfigure}{2.2in}
		\begin{tikzpicture}
		\node at (0,0) {\includegraphics[scale=0.38]{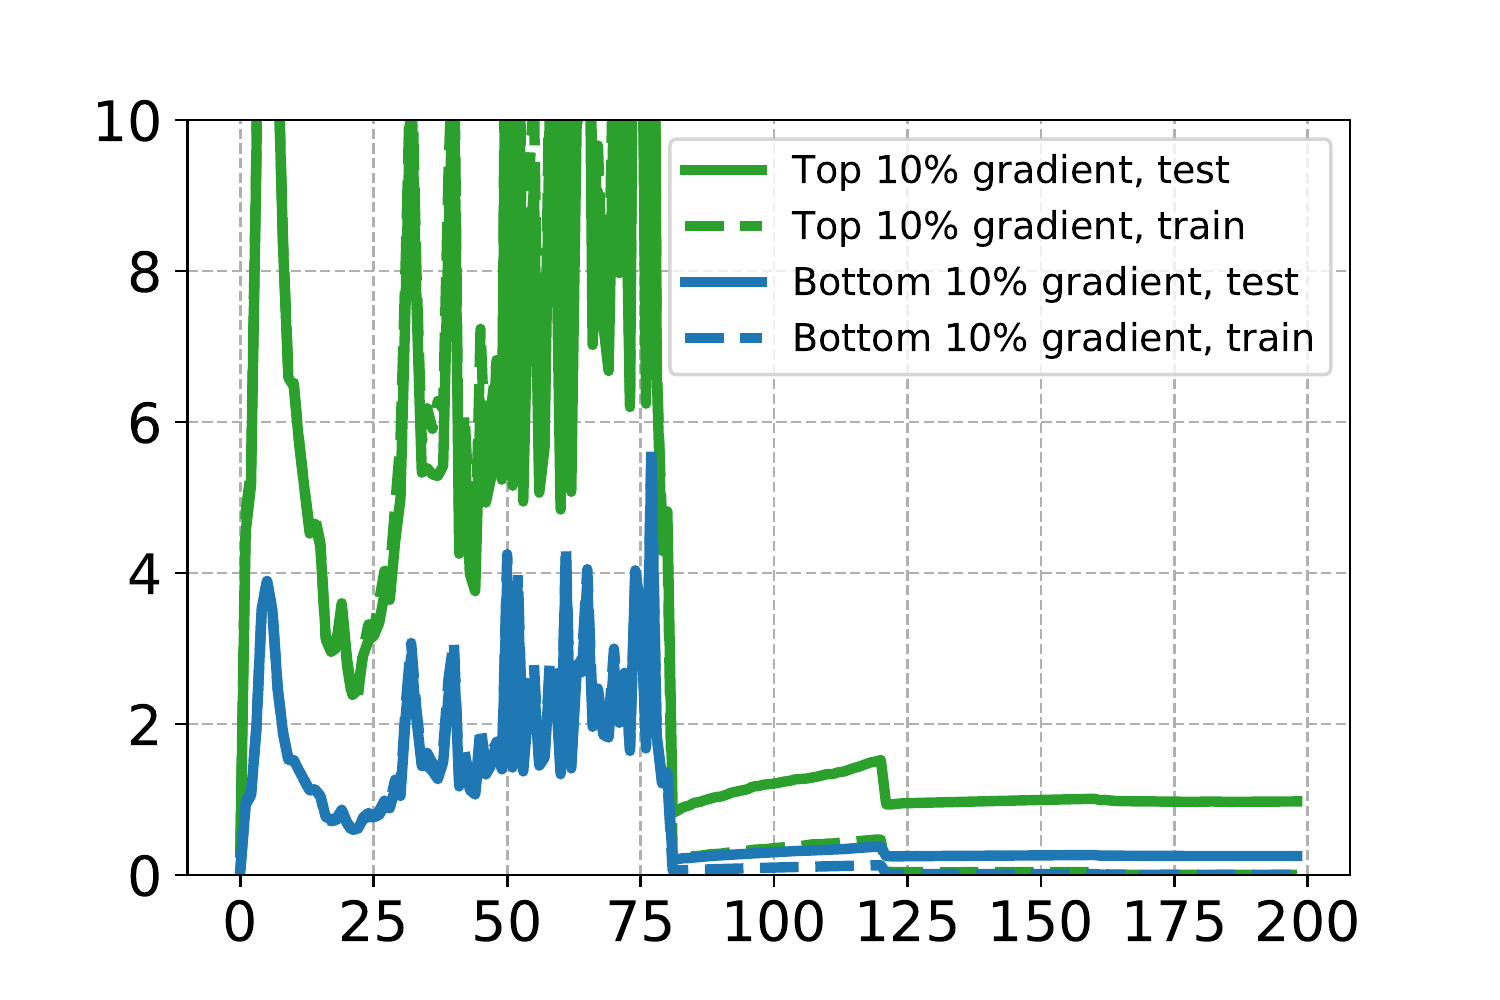}};
		\node at (-3,0) [rotate=90,scale=.8]{$\tn{m\odot\nabla\Lc(\bt_\tau)}^2$};
		\node at (0,-2.1) [scale=.8]{Epoch};
		\end{tikzpicture}\caption{Gradient energy of bottom vs top entries.\\ \quad}\label{fig:app_gradient_fraction_distance_1}
	\end{subfigure}
	\begin{subfigure}{2.2in}
		\begin{tikzpicture}
		\node at (0,0) {\includegraphics[scale=0.38]{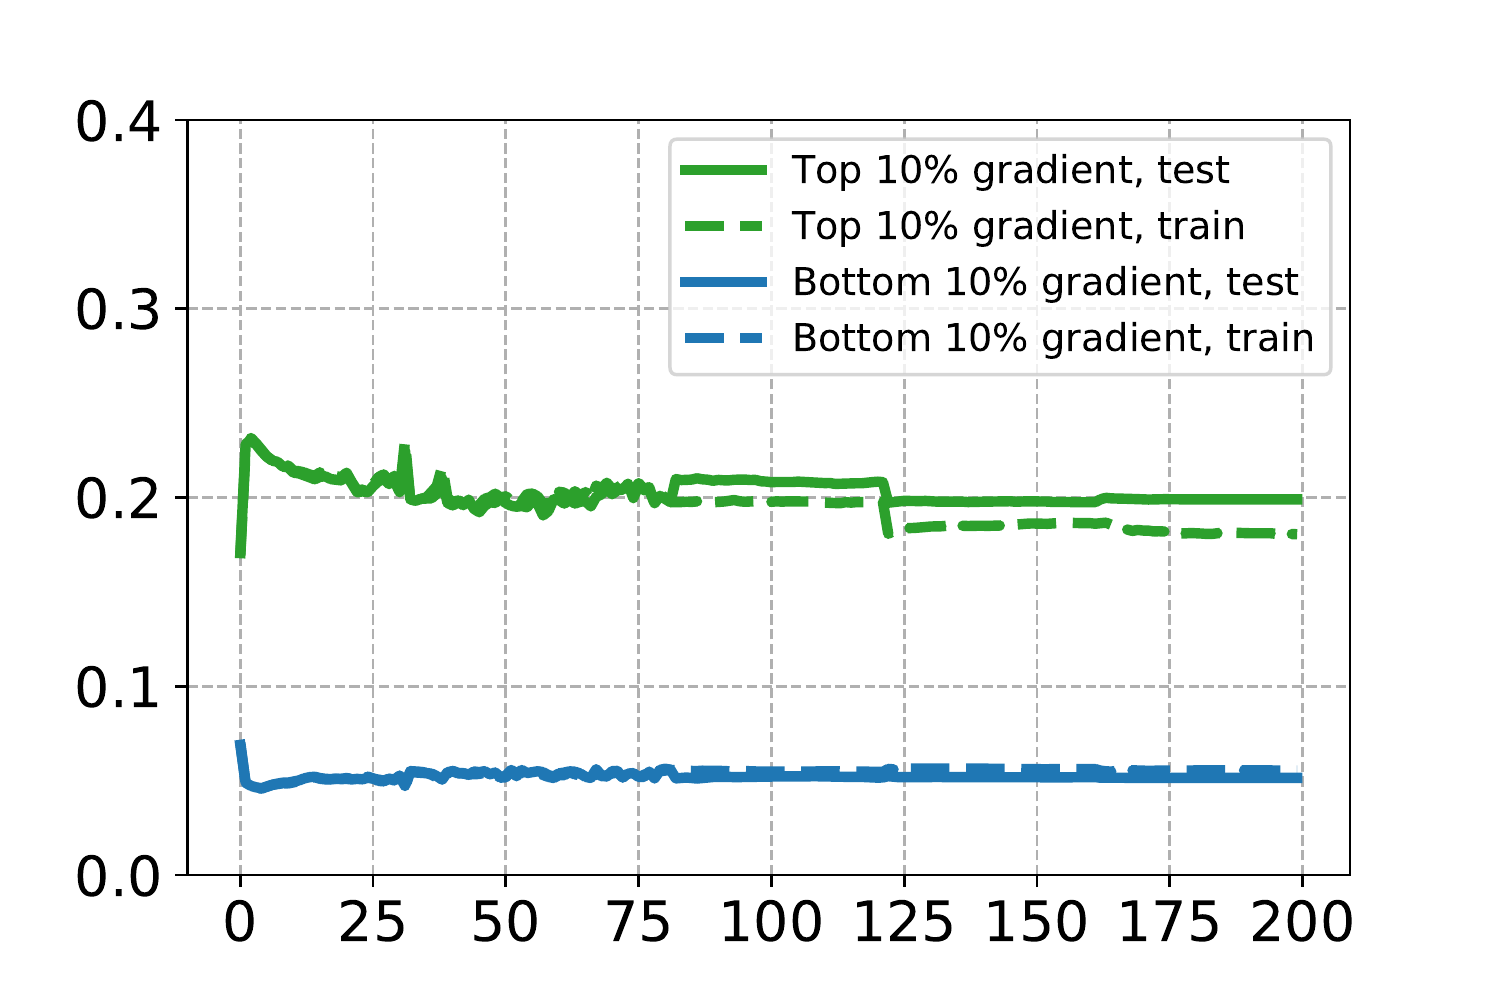}};
		\node at (-3,0) [rotate=90,scale=.8]{Fraction of masked gradient};
		\node at (0,-2.1) [scale=.8]{Epoch};
		\end{tikzpicture}\caption{Fraction of the top/bottom gradient energy.}\label{fig:app_gradient_fraction_distance_2} 
	\end{subfigure}
	\begin{subfigure}{2.2in}
		\begin{tikzpicture}
		\node at (0,0) {\includegraphics[scale=0.38]{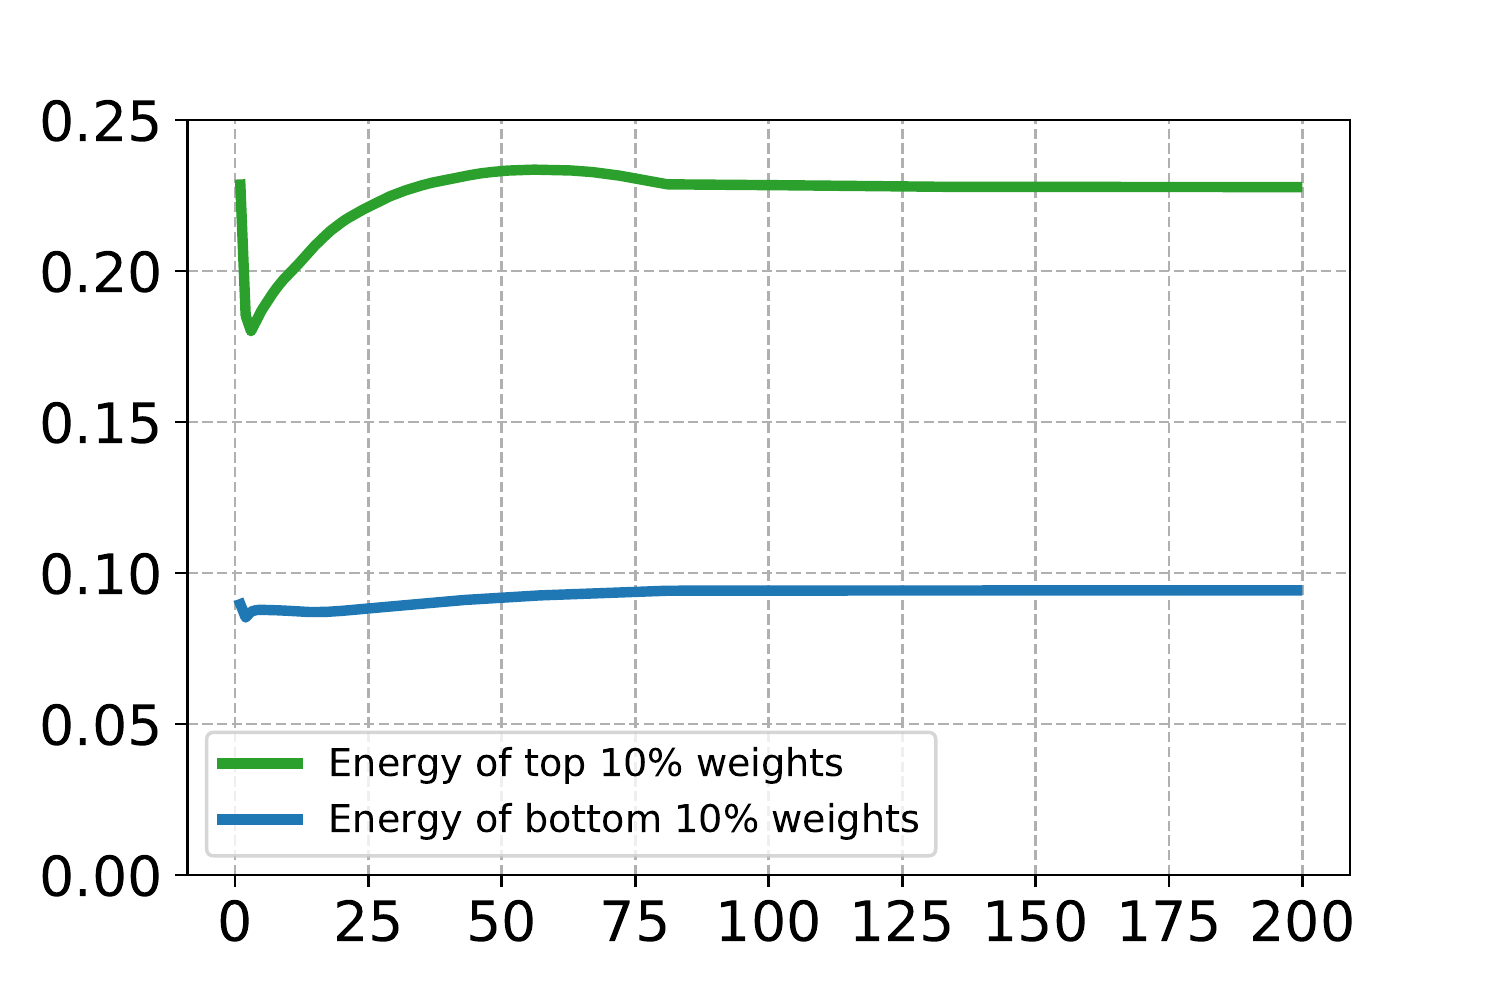}};
		\node at (-3,0) [rotate=90,scale=.8]{Fraction of masked weight};
		\node at (0,-2.1) [scale=.8]{Epoch};
		\end{tikzpicture}\caption{Fraction of the top/bottom weight energy. \\\quad}\label{fig:app_gradient_fraction_distance_3} 
	\end{subfigure}
	\caption{Gradient and weight energy on top and bottom entries, distance pruning. In this figure, we train 10 class ResNet-20 with CIFAR-10 without data augmentation, compute the full gradient of train and test datasets and plot the evolution of the top/bottom 10\% of the gradient and weight using mask $m_{distance}^{10\%}=\text{mask}^{10\%}(\bt_{final}-\bt_0)$. Fig.\ref{fig:app_gradient_fraction_distance_1} and \ref{fig:app_gradient_fraction_distance_2} are same as \ref{fig:gradient_norm} and \ref{fig:gradient_fraction}. Fig.\ref{fig:app_gradient_fraction_distance_3} shows the fraction of masked weight energy $\tn{m\odot\bar{\bt}_{epoch}}^2/\tn{\bar{\bt}_{epoch}}^2$ which are the top and bottom 10\% entries' energy of current weight distances $\bar{\bt}_{epoch}=\bt_{epoch}-\bt_{0}$ }\label{fig:app_gradient_fraction_distance} 
\end{figure*}

\begin{figure*}[t!]
	\begin{subfigure}{2.2in}
		\begin{tikzpicture}
		\node at (0,0) {\includegraphics[scale=0.38]{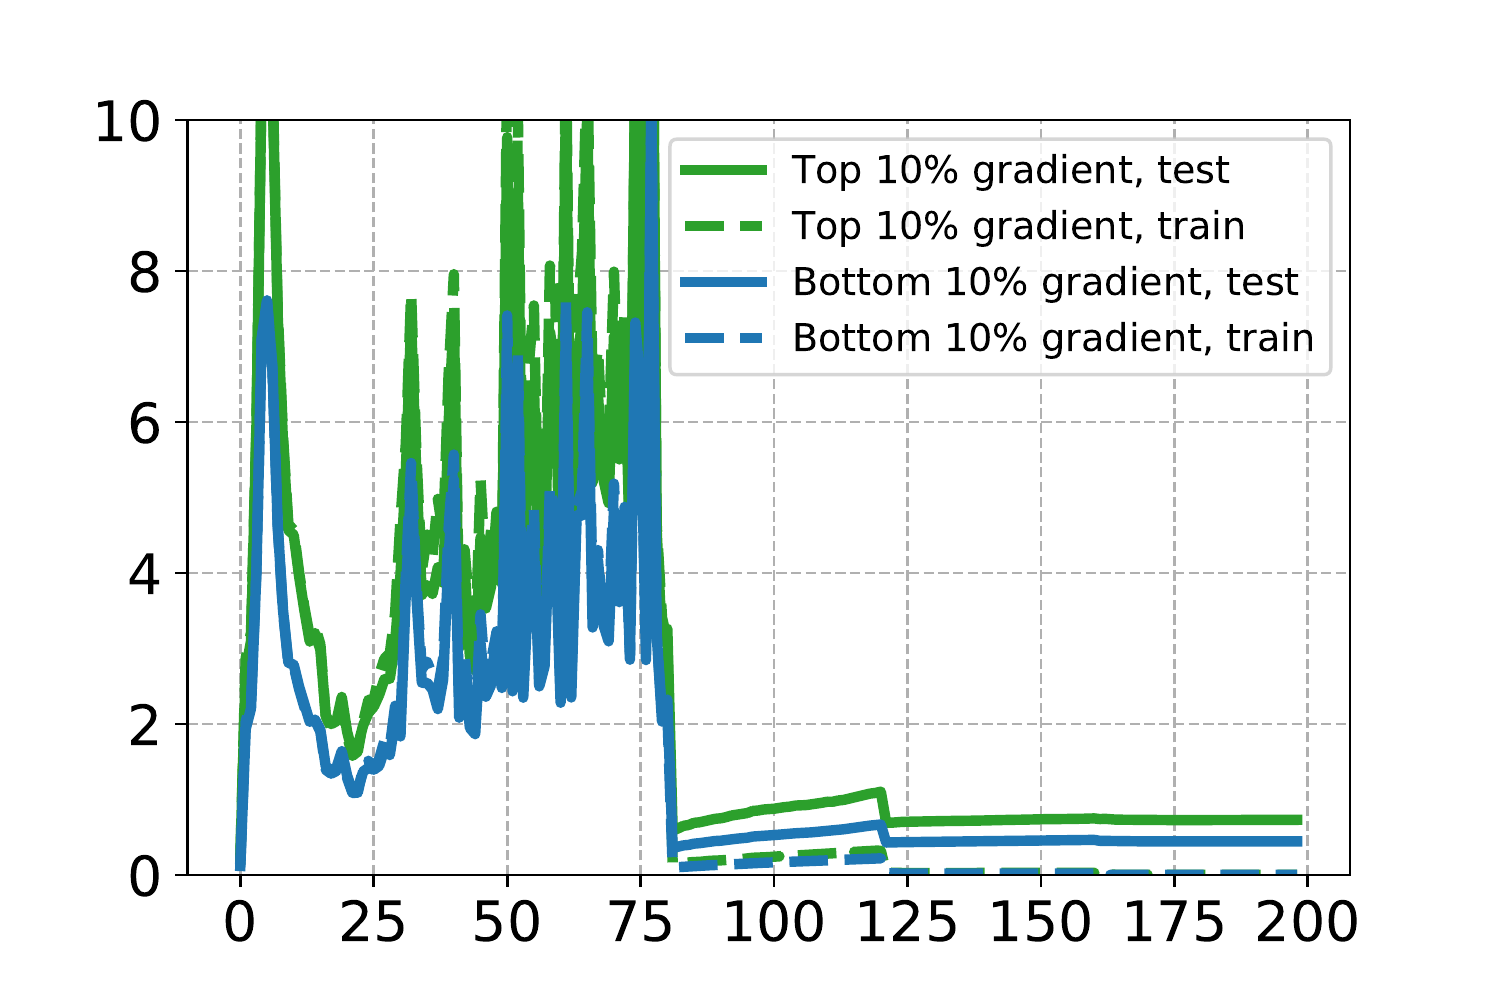}};
		\node at (-3,0) [rotate=90,scale=.8]{$\tn{m\odot\nabla\Lc(\bt_\tau)}^2$};
		\node at (0,-2.1) [scale=.8]{Epoch};
		\end{tikzpicture}\caption{Gradient energy of bottom vs top entries.\\ \quad}\label{fig:app_gradient_fraction_weight_1}
	\end{subfigure}
	\begin{subfigure}{2.2in}
		\begin{tikzpicture}
		\node at (0,0) {\includegraphics[scale=0.38]{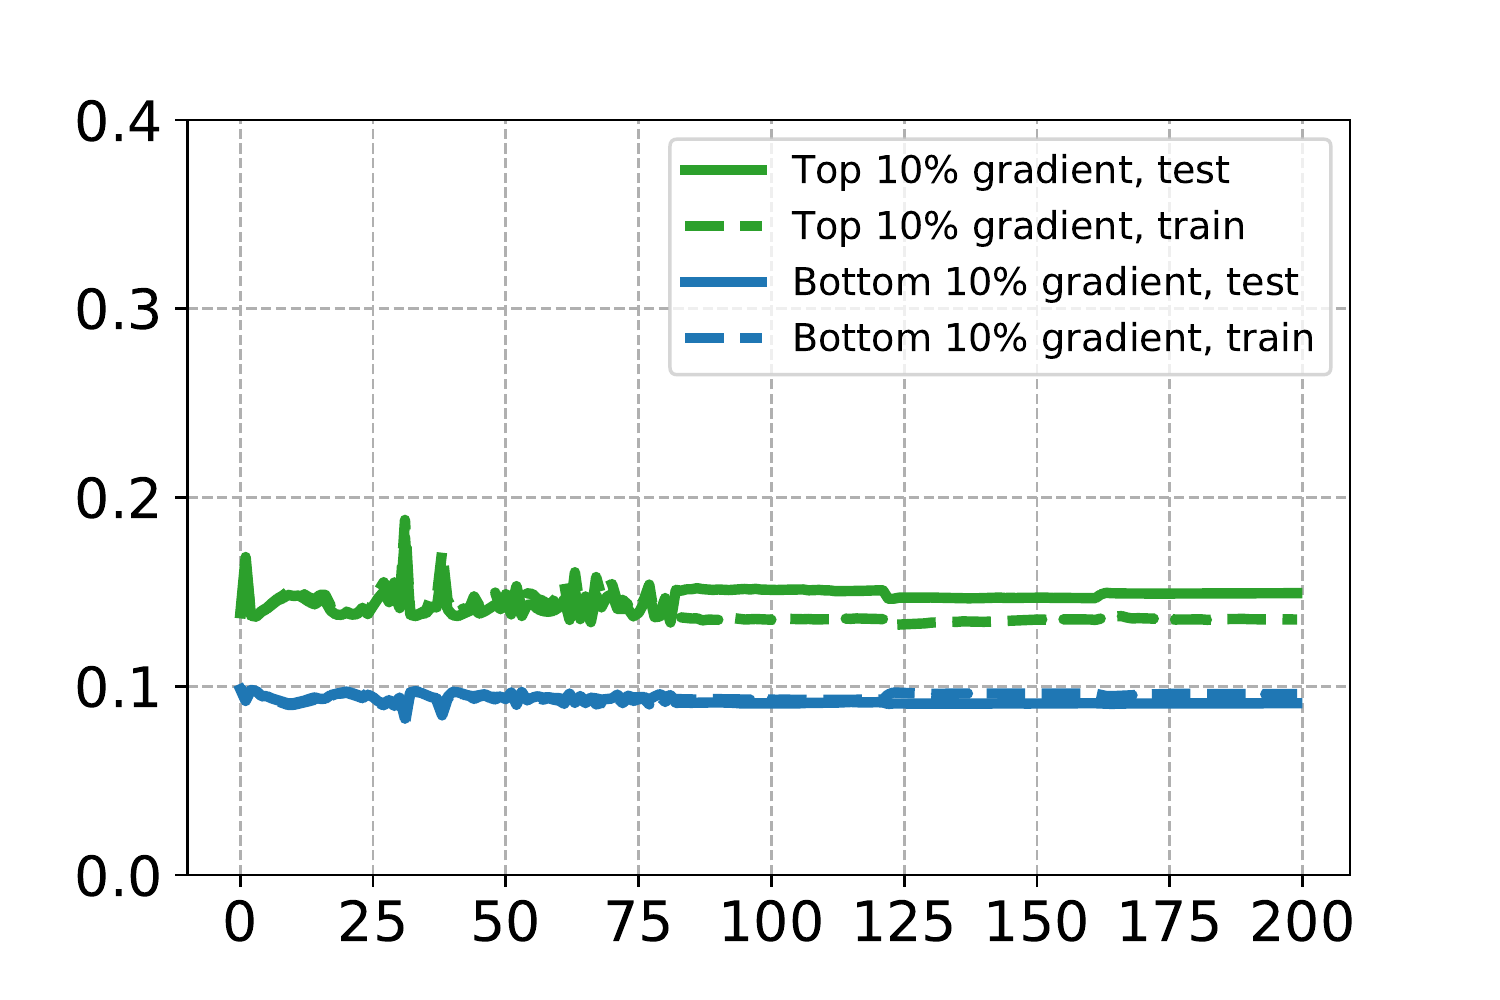}};
		\node at (-3,0) [rotate=90,scale=.8]{Fraction of masked gradient};
		\node at (0,-2.1) [scale=.8]{Epoch};
		\end{tikzpicture}\caption{Fraction of the top/bottom gradient energy.}\label{fig:app_gradient_fraction_weight_2} 
	\end{subfigure}
	\begin{subfigure}{2.2in}
		\begin{tikzpicture}
		\node at (0,0) {\includegraphics[scale=0.38]{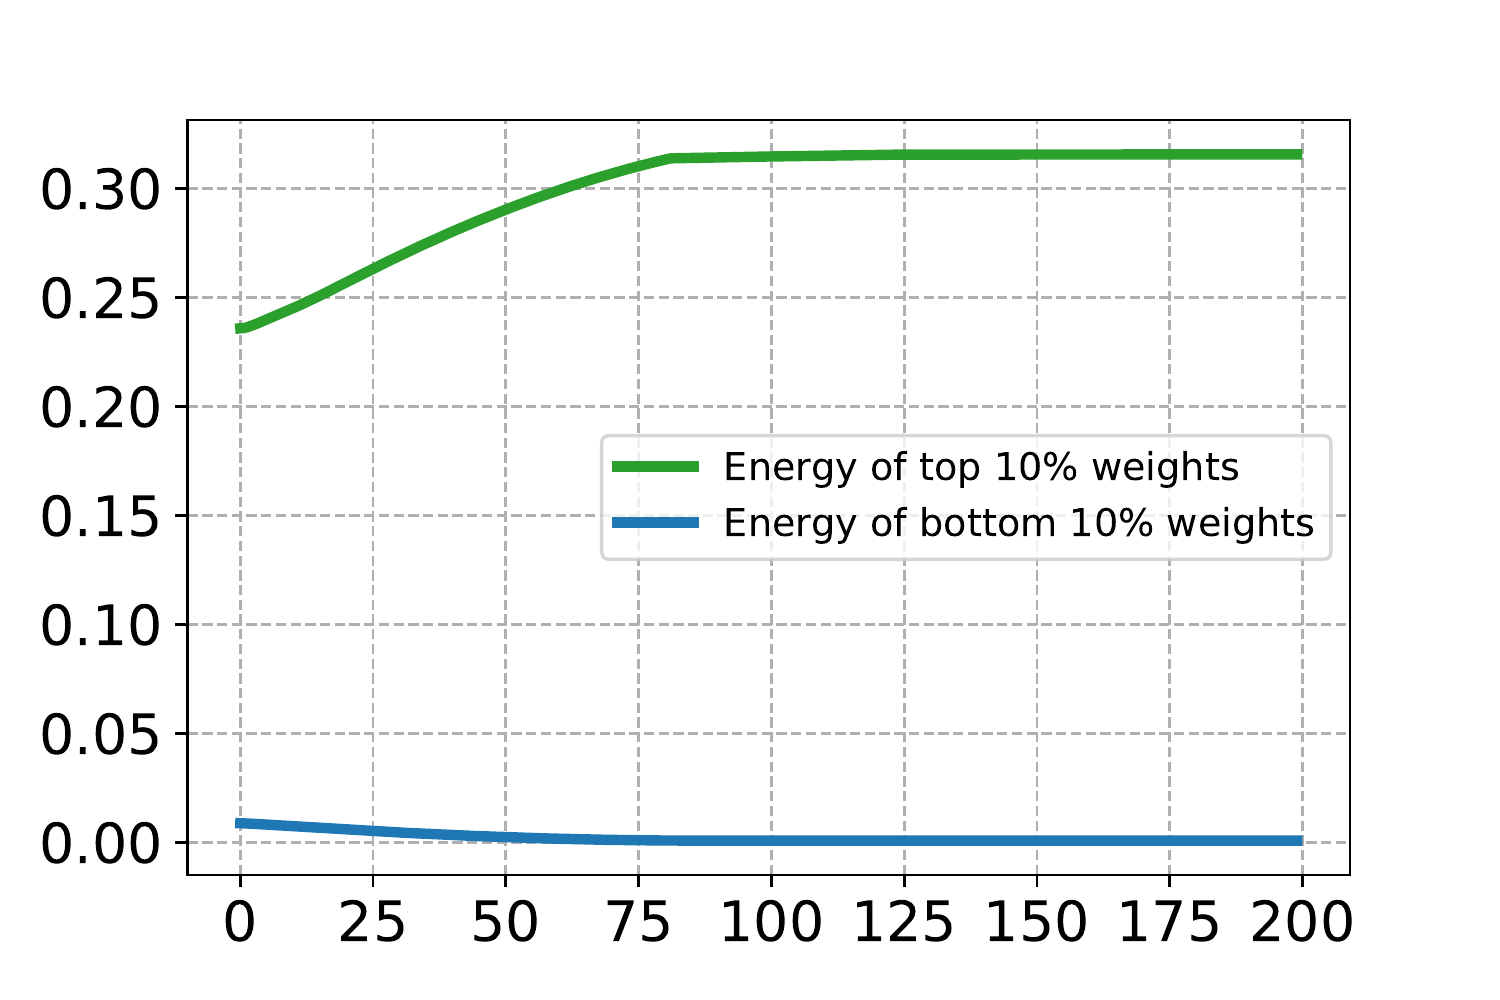}};
		\node at (-3,0) [rotate=90,scale=.8]{Fraction of masked weight};
		\node at (0,-2.1) [scale=.8]{Epoch};
		\end{tikzpicture}\caption{Fraction of the top/bottom weight energy. \\\quad}\label{fig:app_gradient_fraction_weight_3} 
	\end{subfigure}
	\caption{Gradient and weight energy on top and bottom entries, weight pruning. In this figure, we use the same model in Fig.\ref{fig:app_gradient_fraction_distance} but prune the weight by $m_{weight}^{10\%}=\text{mask}^{10\%}(\bt_{final})$. Fig.\ref{fig:app_gradient_fraction_weight_1} and \ref{fig:app_gradient_fraction_weight_2} shows the energy and fraction of masked gradient under weight pruning. Fig.\ref{fig:app_gradient_fraction_weight_3} shows the fraction of masked weight energy $\tn{m_{weight}^{10\%}\odot\bar{\bt}_{epoch}}^2/\tn{\bar{\bt}_{epoch}}^2$ under distance pruning where $\bar{\bt}_{epoch}=\bt_{epoch}-\bt_{0}$}\label{fig:app_gradient_fraction_weight}
\end{figure*}

\subsection{Elastic net on linear regression}
In this section, we provide details in datasets selection and data pre-processing. We firstly select the datasets by the following criterion.
\begin{itemize}
	\item [*] $200\leq$ Number of samples $\leq 100,000$
	\item [*] $10\leq$ Number of features $\leq 4,000$
	\item [*] Number of classes = 2
	\item [*] No missing value
\end{itemize}

Then we discard the feature with more than 10 categories to avoid extremely large dimensions in training datasets (sensitivity test in Table.\ref{table:app_sensitivity_t}) and expand categorical features to one-hot encoding. We standardize the one-hot encoding features to zero mean and unit variance. The labels are also standardized to zero mean and unit variance. We marked that we show the table with geometric mean in Experiment section to mitigate the affection of outliers, but we also provide arithmetic version in Table.~\ref{table:app_lasso_mean}

\begin{table*}[t!]
	\centering
	\begin{adjustbox}{width=\linewidth-0.2in,center}
		\begin{tabular}{*{9}c}
			\toprule
			&  \multicolumn{2}{c}{All datasests, train}&  \multicolumn{2}{c}{All datasests, test}&  \multicolumn{2}{c}{Top 20\%, train} & \multicolumn{2}{c}{Top 20\%, test} \\
			\midrule
			& Correlation    & Accuracy            & Correlation   & Accuracy 	& Correlation    & Accuracy            & Correlation   & Accuracy \\
			Baseline 	&$1.16\pm0.13$  &0.8     &$1.11\pm0.1$  &0.77   &$1.85\pm0.21$ &0.92     &$1.58 \pm0.15$  &0.91 \\
			$\ell_2$ regularization	&$1.41\pm0.15$  &0.8     &$1.35\pm0.14$  &0.77   &$1.95\pm0.22$ &0.92     &$1.67 \pm0.16$  &0.91 \\
			70\% non-zero           &$2.42\pm0.59$  &0.79     &$2.28\pm0.56$  &0.77   &$2.3\pm0.27$ &0.91     &$1.93 \pm0.18$  &0.92 \\
			50\% non-zero          &$2.25\pm0.43$  &0.79     &$2.05\pm0.38$  &0.76   &$2.54\pm0.32$ &0.89     &$2.02 \pm0.16$  &0.89 \\
			20\% non-zero         &$1.97\pm0.26$  &0.77     &$1.76\pm0.19$  &0.75   &$2.79\pm0.36$ &0.87     &$2.1 \pm0.14$  &0.87 \\
			10\% non-zero         &$1.71\pm0.24$  &0.75     &$1.52\pm0.18$  &0.74   &$2.24\pm0.32$ &0.84     &$1.68 \pm0.14$  &0.84 \\
			\bottomrule 
	\end{tabular}\end{adjustbox}\caption{Arithmetic mean of correlations on different sparsity levels of elastic net solutions. Compared to Table.\ref{table:sparsity_level} which used geometric mean, the correlation and error on 70\% and 50\% non-zero are strongly affected by top datasets which have large correlations but geometric mean mitigates this effect gracefully. }\label{table:app_lasso_mean}\vspace{-0.4cm}
	
	%  which indicates the size of powerful features is smaller but more powerful in top performance datasets, which is same as the Fig.~\ref{fig:non-standardized_correlation} where datasets with better performance achieves even higher correlation in sparser model. 
\end{table*}

\begin{table*}[t!]
	\centering
	\begin{adjustbox}{width=\linewidth-0.2in,center}
		\begin{tabular}{*{9}c}
			\toprule
			&  \multicolumn{2}{c}{All datasests, train}&  \multicolumn{2}{c}{All datasests, test}&  \multicolumn{2}{c}{Top 20\%, train} & \multicolumn{2}{c}{Top 20\%, test} \\
			\midrule
			& Correlation    & Accuracy            & Correlation   & Accuracy 	& Correlation    & Accuracy            & Correlation   & Accuracy \\
			Baseline, $t=3$ 	&$0.92\pm0.07$  &0.8     &$0.94\pm0.07$  &0.76   &$1.21\pm0.14$ &0.91     &$1.15 \pm0.12$  &0.91 \\
			Baseline, $t=6$ 	&$0.93\pm0.07$  &0.8     &$0.94\pm0.07$  &0.77   &$1.27\pm0.15$ &0.92     &$1.21 \pm0.13$  &0.91 \\
			Baseline, $t=10$ 	&$0.92\pm0.07$  &0.8     &$0.93\pm0.07$  &0.77   &$1.24\pm0.15$ &0.92     &$1.17 \pm0.12$  &0.91 \\
			Baseline, $t=15$ 	&$0.92\pm0.07$  &0.8     &$0.93\pm0.07$  &0.77   &$1.24\pm0.15$ &0.92     &$1.17 \pm0.12$  &0.91 \\
			Baseline, $t=20$ 	&$0.92\pm0.07$  &0.8     &$0.93\pm0.07$  &0.77   &$1.24\pm0.15$ &0.92     &$1.17 \pm0.12$  &0.91 \\
			
			\midrule
			$\ell_2$ regularization, $t=3$	&$1.11\pm0.09$  &0.8     &$1.08\pm0.09$  &0.77   &$1.3\pm0.16$ &0.91     &$1.21 \pm0.14$  &0.91 \\
			$\ell_2$ regularization, $t=6$  &$1.11\pm0.09$  &0.8     &$1.09\pm0.09$  &0.77   &$1.34\pm0.16$ &0.92     &$1.25 \pm0.14$  &0.91 \\
			$\ell_2$ regularization, $t=10$ &$1.11\pm0.09$  &0.8     &$1.08\pm0.09$  &0.77   &$1.29\pm0.16$ &0.92     &$1.19 \pm0.13$  &0.91 \\
			$\ell_2$ regularization, $t=15$	&$1.11\pm0.09$  &0.8     &$1.08\pm0.09$  &0.77   &$1.29\pm0.16$ &0.92     &$1.19 \pm0.13$  &0.91 \\
			$\ell_2$ regularization, $t=20$	&$1.11\pm0.09$  &0.8     &$1.08\pm0.09$  &0.77   &$1.29\pm0.16$ &0.92     &$1.19 \pm0.13$  &0.91 \\
			
			\midrule
			70\% non-zero, $t=3$        &$1.32\pm0.15$  &0.79     &$1.27\pm0.14$  &0.77   &$1.43\pm0.2$ &0.91     &$1.32 \pm0.16$  &0.91 \\
			70\% non-zero, $t=6$        &$1.33\pm0.15$  &0.79     &$1.28\pm0.14$  &0.77   &$1.47\pm0.2$ &0.91     &$1.36 \pm0.17$  &0.92 \\
			70\% non-zero, $t=10$        &$1.34\pm0.15$  &0.79     &$1.29\pm0.14$  &0.77   &$1.45\pm0.2$ &0.91     &$1.33 \pm0.17$  &0.92 \\
			70\% non-zero, $t=15$        &$1.34\pm0.15$  &0.79     &$1.29\pm0.14$  &0.77   &$1.45\pm0.2$ &0.91     &$1.33 \pm0.17$  &0.92 \\
			70\% non-zero, $t=20$        &$1.34\pm0.15$  &0.79     &$1.29\pm0.14$  &0.77   &$1.45\pm0.2$ &0.91     &$1.33 \pm0.17$  &0.92 \\

			\midrule
			50\% non-zero, $t=3$        &$1.44\pm0.14$  &0.78     &$1.36\pm0.12$  &0.76   &$1.8\pm0.17$ &0.89     &$1.64 \pm0.13$  &0.89 \\
			50\% non-zero, $t=6$        &$1.44\pm0.14$  &0.79     &$1.37\pm0.12$  &0.76   &$1.89\pm0.17$ &0.89     &$1.73 \pm0.13$  &0.89 \\
			50\% non-zero, $t=10$        &$1.45\pm0.14$  &0.79     &$1.37\pm0.13$  &0.76   &$1.84\pm0.18$ &0.89     &$1.66 \pm0.13$  &0.89 \\
			50\% non-zero, $t=15$        &$1.45\pm0.14$  &0.79     &$1.37\pm0.13$  &0.76   &$1.84\pm0.18$ &0.89     &$1.66 \pm0.13$  &0.89 \\
			50\% non-zero, $t=20$        &$1.45\pm0.14$  &0.79     &$1.37\pm0.13$  &0.76   &$1.84\pm0.18$ &0.89     &$1.66 \pm0.13$  &0.89 \\

			\midrule
			20\% non-zero, $t=3$        &$1.5\pm0.12$  &0.76     &$1.4\pm0.1$  &0.75   &$2.06\pm0.19$ &0.87     &$1.79 \pm0.13$  &0.87 \\
			20\% non-zero, $t=6$        &$1.5\pm0.12$  &0.77     &$1.41\pm0.1$  &0.75   &$2.18\pm0.19$ &0.87     &$1.9 \pm0.14$  &0.87 \\
			20\% non-zero, $t=10$        &$1.51\pm0.12$  &0.77     &$1.41\pm0.1$  &0.75   &$2.06\pm0.19$ &0.87     &$1.79 \pm0.13$  &0.87 \\
			20\% non-zero, $t=15$        &$1.51\pm0.12$  &0.77     &$1.41\pm0.1$  &0.75   &$2.06\pm0.19$ &0.87     &$1.79 \pm0.13$  &0.87 \\
			20\% non-zero, $t=20$        &$1.51\pm0.12$  &0.77     &$1.41\pm0.1$  &0.75   &$2.06\pm0.19$ &0.87     &$1.79 \pm0.13$  &0.87 \\

			\midrule
			10\% non-zero, $t=3$       &$1.23\pm0.13$  &0.74     &$1.15\pm0.12$  &0.73   &$1.54\pm0.14$ &0.83     &$1.36 \pm0.1$  &0.84 \\
			10\% non-zero, $t=6$       &$1.23\pm0.13$  &0.75     &$1.16\pm0.12$  &0.74   &$1.62\pm0.14$ &0.84     &$1.45 \pm0.11$  &0.85 \\
			10\% non-zero, $t=10$       &$1.24\pm0.13$  &0.75     &$1.16\pm0.12$  &0.74   &$1.58\pm0.15$ &0.84     &$1.39 \pm0.1$  &0.84 \\
			10\% non-zero, $t=15$       &$1.24\pm0.13$  &0.75     &$1.16\pm0.12$  &0.74   &$1.58\pm0.15$ &0.84     &$1.39 \pm0.1$  &0.84 \\
			10\% non-zero, $t=20$       &$1.24\pm0.13$  &0.75     &$1.16\pm0.12$  &0.74   &$1.58\pm0.15$ &0.84     &$1.39 \pm0.1$  &0.84 \\

			\bottomrule 
	\end{tabular}\end{adjustbox}\caption{Sensitivity test for threshold selection. We discard a categorical feature when it has more than $t$ categories. The correlation and accuracy on different sparsity levels of elastic net solutions which are showed in the table indicates that the value of $t$ does not affect result when $t$ is larger than 10. }\label{table:app_sensitivity_t}\vspace{-0.4cm}
	
	%  which indicates the size of powerful features is smaller but more powerful in top performance datasets, which is same as the Fig.~\ref{fig:non-standardized_correlation} where datasets with better performance achieves even higher correlation in sparser model. 
\end{table*}
