# Supplementary material for: Exploring Weight Importance and Hessian Bias in Model Pruning
Source: arXiv:2006.10903 source file (2020-06-19)
Supplement: Supplementary file 3 [file appendix_improve.tex]

\section{Proof of Lemma \ref{lemma:better acc with la}}
\begin{lemma}[Monotonic Improvement with Implicit Bias]~\label{lemma:better acc with la} Suppose $\btb$ is a sparse ground-truth vector whose nonzero entries are subset of $\Delta\subset[p]$. Suppose labels obey $\y=\x^T\btb$ and $\bSi=\Iden_p$. Suppose $n>|\Delta|$ and the submatrix induced by the columns of $\X$ indexed by $\Delta$ is full-rank. Consider diagonal matrices $\La:=\La(\la)\in\R^{p\times p}$ where $\La_{i,i}=\la$ if $i\in \Delta$ and $\La_{i,i}=1$ otherwise. Let $\bth^\la=\bth^{\La(\la)}$ be the minima of empirical risk. Define the associated population risk $\Lc_\la=\Lc_{\La(\la)}(\bth^\la)$. Then, $\Lc_\la$ is strictly decreasing function of $\la$ and $\lim_{\la\rightarrow\infty}\Lc_\la=0$.
\end{lemma}
\begin{proof}
Set $s=|\Delta|$. Without losing generality, assume $\Delta$ is the first $s$ entries of $\bt=[\bt_1~\bt_2]$. Also decompose $\X=[\X_1~\X_2]$ where $\X_1\in\R^{n\times s}$. Observe that
\begin{align}
\bth^\la&=\arg\min_{\bt}\tn{\bt}^2\quad\text{subject to}\quad \X\btb=\X_\la \bt=\la\X_1\bt_1+\X_2\bt_2\\
&=\arg\min_{\bt}\tn{\bt_1}^2+\tn{\bt_2}^2\quad\text{subject to}\quad \X_1(\la\bt_1-\btb_1)+\X_2\bt_2=0\\
\La\bth^\la&=\arg\min_{\bt}\la^{-2}\tn{\bt_1}^2+\tn{\bt_2}^2\quad\text{subject to}\quad \X_1(\bt_1-\btb_1)+\X_2\bt_2=0\\
\La\bth^\la-\btb&=\arg\min_{\vb}\tn{\btb_1+\vb_1}^2+\la^2\tn{\vb_2}^2\quad\text{subject to}\quad \X_1\vb_1+\X_2\vb_2=0,\\
&=\arg\min_{\alpha\vb}\tn{\btb_1+\alpha\vb_1}^2+\alpha^2\la^2\tn{\vb_2}^2\quad\text{subject to}\quad \X_1\vb_1+\X_2\vb_2=0,~\tn{\vb}=1,~\alpha\geq 0\nn\\
&:=\arg\min_{\alpha\vb}\Lc_\la(\alpha,\vb)\quad\text{subject to}\quad \X_1\vb_1+\X_2\vb_2=0,~\tn{\vb}=1,~\alpha\geq 0.
\end{align}
$\La\bth^\la-\btb$ is exactly the quantity of interest for test loss. Let $\vb_\la,\alpha_\la=\alpha_\la(\vb_\la)$ be the optimal pair for a fixed $\la$. Then, test loss is simply $\alpha_\la^2$. To proceed, fixing $\vb$ and differentiating with respect to $\la$, we can optimize $\alpha$ as follows
\begin{align}
0.5\frac{\pa}{\pa\alpha}\Lc_\la(\alpha,\vb)&=\vb_1^T(\btb_1+\alpha\vb_1)+\alpha\la^2\tn{\vb_2}^2\\
&=\vb_1^T\btb_1+\alpha (\tn{\vb_1}^2+\la^2\tn{\vb_2}^2)\implies \alpha_\la(\vb)=\frac{-\vb_1^T\btb_1}{\tn{\vb_1}^2+\la^2\tn{\vb_2}^2}.
\end{align}
Observe that, by definition $\vb$ is a null space element and $\vb_1^T\btb_1$ is non-positive (otherwise it would violate min-norm). Since $\X_{\Delta}$ is full-rank, $\X_{\Delta}\vb_1\neq 0$ and there exists some $\eps>0$ such that $\tn{\vb_2}\geq \eps$. We then have that
\[
\lim_{\la\rightarrow \infty}\alpha_\la=\lim_{\la\rightarrow\infty}\frac{-\vb_{\la,1}^T\btb_1}{\tn{\vb_{\la,1}}^2+\la^2\tn{\vb_{\la,2}}^2}\leq \lim_{\la\rightarrow\infty}\frac{\tn{\btb}}{1+(\la^2-1)\eps^2}=0.
\]
Thus, as $\la$ grows, the test error goes to zero as advertised. What remains is showing the strict monotonicity. Fix $\kappa>\la$. We will show that $\alpha_\kappa<\alpha_\la$. 
%First note that $\vb_\kappa,\alpha_\kappa$ minimizes
%\[
%\min_{\alpha\vb}\tn{\btb_1+\alpha\vb_1}^2+\alpha^2\kappa^2\tn{\vb_2}^2\quad\text{subject to}\quad \X\vb=0,\tn{\vb}=1,~\alpha\geq 0.
%\]
%Now, let us suppose $\alpha_\la\leq \alpha_\kappa$ and obtain a contradiction.
Fix $\vb_\la,\vb_\kappa$. Given $\vb$, define the critical quantities $a=-\vb_1^T\btb_1$ and $b=\tn{\vb_2}^2$. We have that $\alpha_{\la}(\vb)=\frac{a}{1+(\la^2-1)b}$. Let $(a_\la,b_\la),(a_\kappa,b_\kappa)$ be these quantities for $\vb_\la,\vb_\kappa$ respectively. Substituting, the loss takes the form
\begin{align}
\Lc_\la(\alpha,\vb)-\tn{\btb}^2&=2\alpha\vb_1^T\btb+\alpha^2(\tn{\vb_1}^2+\la^2\tn{\vb_2}^2)\\
&=-2\alpha a+\frac{a^2}{(1+(\la^2-1)b)^2}(1+(\la^2-1)b)\\
&=\frac{-a^2}{1+(\la^2-1)b}.
\end{align}
Next, observe the facts that $\Lc_\la(\alpha_\la,\vb_\la)< \Lc_\la(\alpha_\la(\vb_\kappa),\vb_\kappa)$ and $\Lc_\kappa(\alpha_\kappa,\vb_\kappa)< \Lc_\la(\alpha_\kappa(\vb_\la),\vb_\la)$. Strict inequalities are due to strong convexity of the loss i.e.~the equality would violate the optimality of $\vb_\la$ by constructing a strictly better solution via convex combination (and similarly $\vb_\kappa$).
\begin{align}
&\frac{a_\la^2}{1+(\la^2-1)b_\la}> \frac{a_\kappa^2}{1+(\la^2-1)b_\kappa}\\
&\frac{a_\kappa^2}{1+(\kappa^2-1)b_\kappa}> \frac{a_\lambda^2}{1+(\kappa^2-1)b_\lambda}.
\end{align}
This leads to
\[
\frac{1+(\kappa^2-1)b_\lambda}{1+(\kappa^2-1)b_\kappa}> \frac{a_\lambda^2}{a_\kappa^2}>\frac{1+(\la^2-1)b_\la}{1+(\la^2-1)b_\kappa}>\frac{1+(\la^2-1)b_\la}{1+(\kappa^2-1)b_\kappa},
\]
where the last inequality follows from $\kappa>\la$ and $b_\kappa>0$. This yields the target relation
\[
\frac{a_\la^2}{1+(\la^2-1)b_\la}>\frac{a_\kappa^2}{1+(\kappa^2-1)b_\kappa}\iff \alpha_\la>\alpha_\kappa.
\]
%Combining and using $\kappa>\la$, we find
%\begin{align}
%\frac{1+(\la^2-1)b_\la}{1+(\la^2-1)b_\kappa}\leq \frac{1+(\kappa^2-1)b_\la}{1+(\kappa^2-1)b_\kappa}\implies b_\la\geq b_\kappa.
%\end{align}
%This also implies $a_\la\geq a_\kappa$. Consequently
%\[
%\alpha_\la=\frac{a_\la}{1+(\la^2-1)b_\la}\geq  \frac{a_\kappa}{1+(\la^2-1)b_\kappa}
%\]
%\begin{align}
%\alpha_\kappa=\alpha_\kappa(\vb_\kappa)<\alpha_\lambda(\vb_\kappa)
%\end{align}
%\begin{align}
%\Lc_\kappa(\alpha_\kappa,\vb_\lambda)&\geq \Lc_\kappa(\alpha_\kappa,\vb_\kappa)\\
%&> \Lc_\lambda(\alpha_\kappa,\vb_\kappa)\\
%&\geq \Lc_\lambda(\alpha_\lambda,\vb_\lambda).
%\end{align}
\end{proof}
