# Supplementary material for: Exploring Weight Importance and Hessian Bias in Model Pruning
Source: arXiv:2006.10903 source file (2020-06-19)
Supplement: Supplementary file 4 [file appendix_random.tex]

\section{Proofs of Gaussian Width Results}
\subsection{Proof of Lemma \ref{thm spike}}
\begin{proof} Let us characterize the colored tangent cone defined as
\[
\Tc_R=\{\bSi_R^{1/2}\w\bgl \w\in\Tc\}.
\]
Denote the set of nonzero coordinates of $\bt$ by $S$ and its complement by $S^c$. Using symmetry of the null space property, without losing generality, we can assume that the first $s$ coordinates of $\bt_\st$ are strictly positive. Given any $\w'\in \Tc_R$, we can set $\w'=\bSi_R^{1/2}\w$, which yields
\[
\w'=\w+\frac{R-1}{s}\onebb\onebb^T\w_S\quad\text{where}\quad \onebb^T\w_S+\tone{\w_{S^c}}\leq 0
\]
This implies that $\onebb^T\w'_S=R\onebb^T\w_S$ and $\w'_{S^c}=\w'_S$ so that
\[
\frac{\onebb^T}{R}\w'_S+\tone{\w'_{S^c}}=\onebb^T\w_S+\tone{\w_{S^c}}\leq 0.
\]
Following this, define the weighted-$\ell_1$ subdifferential set 
\[
\pa_R=\{\g\bgl \g_S=\frac{\onebb^T}{R}~~\text{and}~~\tin{\g_{S^c}}\leq 1\}.
\]
Observe that, for any $\g\in \pa_R,\w'\in\Tc_R$, we have that $\g^T\w'\leq 0$. Hence $\pa_R$ is subset of the polar cone of $\Tc_R$ denoted by $\Tc_R^\circ$.

%$\g_S=\alpha\onebb+\vb$ where $\vb\in \onebb^c$ and $\tn{\vb}\leq \dots$ and $\tin{\g_{S^c}}\leq R$.
%\[
%\g^T\w=\g_S^T\w_S+\g_S^T\frac{R-1}{s}\onebb\onebb^T\w_S+\g_{S^c}^T\w_{S^c}\leq \beta\tn{\w_S}+\alpha R\onebb^T\w_S+R\tone{\w_{S^c}}
%\]
\begin{comment}
$\g_S=\alpha\onebb+\vb$ where $\vb\in \onebb^c$ and $\tn{\vb}\leq \dots$ and $\tin{\g_{S^c}}\leq R$.
\[
\g^T\w=\g_S^T\w_S+\g_S^T\frac{R-1}{s}\onebb\onebb^T\w_S+\g_{S^c}^T\w_{S^c}\leq \beta\tn{\w_S}+\alpha R\onebb^T\w_S+R\tone{\w_{S^c}}
\]
\end{comment}

Now let $\h\sim\Nn(0,\Iden)$. From duality, it follows that, for any choice of $\la>0$ \cite{chandrasekaran2012convex}
\[
\sup_{\w'\in\Tc_R,\tn{\w'}\leq 1} \w'^T\h\leq \text{dist}(\h, \Tc_R^\circ)\leq \text{dist}(\h, \la\pa_R).
\]
Taking expectations, this yields
\[
\omega_R(\Tc)^2\leq \E[\tn{\h,\la\pa_R}^2]:=\Dc_\la.
\]
To proceed, we will obtain small $\Dc_\la$ by picking proper $\la$ values. We make use of the following bound from \cite{chandrasekaran2012convex}.
%\begin{lemma} 
\begin{align}
\E_{g\sim\Nn(0,1)}[\shr{\la}{g}^2]\leq \sqrt{\frac{2}{\pi}}\frac{1}{\la}\e^{-\la^2/2}.%\sqrt{2/\pi}\e^{-\la^2/2}.
\end{align}
%To proceed, we have
The distance over the off-support entries $S^c$ is given by $\shr{\la}{h_i}$ and on-support entries are simply $h_i-1/R$. Hence, we find
\[
\Dc_\la\leq s(1+\la^2/R^2)+(p-s)\sqrt{\frac{2}{\pi}}\frac{1}{\la}\e^{-\la^2/2}.
\]
%Optimize right hand side by differentiating over $\la$ to find
We pick $\la$ to keep the $(p-s)\sqrt{\frac{2}{\pi}}\frac{1}{\la}\e^{-\la^2/2}$ term small. Setting $\la=\sqrt{2\log(p/s)}$ leads to the bound
\[
\Dc_\la\leq s(1+\la^2/R^2)+s/2\leq s(\frac{3}{2}+\frac{2\log(p/s)}{R^2})
\]
Setting the larger value $\la=\sqrt{2\log(p)}$ yields
\[
\Dc_\la\leq s(1+\la^2/R^2)+1\leq s(1+\frac{2\log(p)}{R^2})+1
\]
Together, these imply
\[
\omega_R(\Tc)^2\leq \min(s(1+\frac{2\log(p)}{R^2})+1, s(\frac{3}{2}+\frac{2\log(p/s)}{R^2})).
\]
\end{proof}

\subsection{Proof of Theorem \ref{cov gen thm}}

\begin{proof} Set $\bSi'=\frac{R-1}{s}\s\s^T+\bSi_{\text{tail}}$ and $\bSi''=\frac{R-1}{s}\s\s^T+\Iden_p$. Apply Lemma \ref{additive lem} and \ref{low rank lem} to find that
\begin{align}
\omega_{\bSi}(T)\leq \omega_{\bSi'}(T)+ \omega_{\bSi_{LR}}(T)\leq \omega_{\bSi'}(T)+\sqrt{d}.
\end{align}
Next, we apply Lemma \ref{condition lem} to obtain $\omega_{\bSi'}(T)\leq \sqrt{\kappa}\omega_{\bSi''}(T)$. Finally, use Lemma \ref{thm spike} to obtain
\[
\omega_{\bSi}(T)\leq \sqrt{\kappa s(\frac{3}{2}+\frac{2\log(p/s)}{R^2})}+\sqrt{d}.
\]
We conclude by applying Lemma \ref{gordon sample}.
\end{proof}

\subsection{Results on Gaussian Width Analysis}
\begin{comment}
\begin{lemma} Let $\Tc$ be the $\ell_1$ tangent cone. We have that
\[
\omega_{\bSi}(\Tc)\leq.
\]
\end{lemma}
\begin{proof} Fix $\g$ and let $\Cc=(\bSi\Tc)^{o}$. Observe that
\[
\sup_{\vb\in \bSi\Tc}\vb^T\g=\tn{\g-\Pi_{\Cc}(\g)}
\]
Next, we find a subset of $\Cc$ as follows. Suppose $\ub$ satisfies $\ub^T\vb\leq 0$ for all $\vb\in\Tc$. Then $(\bSi^{-1}\ub)^T(\bSi\vb)\leq 0$ as well hence $\bSi^{-1}\ub\in\Cc$. Hence $\Cc=\bSi^{-1}\Tc^{o}$. Suppose $\ub\in \Cc$ be the closest to $\g$. Then
\[
\tn{\g-\ub}=\tn{\bSi^{-1}\bSi(\g-\ub)}
\]
Threshold the off-support terms $(\bSi\g)_{S^c}$ by using the fact that each of these are Gaussian with variance bounded by $1$.
\end{proof}
Let $\g\sim\Nn(0,\Iden_p)$. Consider
\[
\sup_{\vb\in\Tc} \frac{\g^T\bSi\vb}{\tn{\bSi\vb}}
\]
Let $\|\bSi\|\leq 1$.
\[
\w'=\w_S+\bSi\w_{S^c}\implies \onebb^T\w_S+(\g^T\bSi^{-1})\bSi\w_{S^c}\leq 0?
\]
Subgradient set is given by $[\onebb~\bSi^{-1}\g]$. Use the fact that $\bSi^{-1}\g$ has small $\ell_\infty$ norm to bound the covariance using standard tricks (achieves $\log p$ instead of $\log (p/n)$).
\end{comment}
\begin{lemma}[Subadditive Gaussian Width] \label{additive lem}Let $\g\distas\Nn(0,\Iden_p)$ and $(\bSi_i)_{i=1}^K\subset\R^{p\times p}$ be positive semi-definite matrices and set $\bSi=\sum_{i=1}^K\bSi_i$. Then,%,\subset\Bc^{d}$% where $\bSi_i=\Ub\La_i\Ub^T$
\[
\omega_{\bSi}(\Cc)\leq \sum_{i=1}^K\omega_{\bSi_i}(\Cc).%+\omega_{\bSi_2}(\Cc)
\]
\end{lemma}
\begin{proof} Let $\g,(\g_i)_{i=1}^K\distas\Nn(0,\Iden_p)$ be independent vectors. Observe that $\bSi^{1/2}\g\sim \sum_{i=1}^K\bSi_i^{1/2}\g_i$. Using the fact that $\w^T\bSi\w\geq \w^T\bSi_i\w$ for all $1\leq i\leq K$, we find that
\begin{align*}
\E[\sup_{\w\in\Tc}\frac{\g^T\bSi^{1/2}\w}{\tn{\bSi^{1/2}\w}}]&=\E[\sup_{\w\in\Tc}\frac{\g_i^T\sum_{i=1}^K\bSi_i^{1/2}\w}{\tn{\bSi^{1/2}\w}}]\\
&\leq \E[\sup_{\w\in\Tc}\frac{\g_i^T\sum_{i=1}^K\bSi_i^{1/2}\w}{\tn{\bSi_i^{1/2}\w}}]\\
&\leq \sum_{i=1}^K\E[\sup_{\w\in\Tc}\frac{\g_i^T\bSi_i^{1/2}\w}{\tn{\bSi_i^{1/2}\w}}]\\
&=\sum_{i=1}^K\omega_{\bSi_i}(\Tc)
%\sim\sup_{\w\in\Ub\Tc}\frac{\g^T\La^{1/2}\w}{\tn{\La^{1/2}\w}}=\sup_{\w\in\Ub\Tc}\frac{\g_1^T\La_1^{1/2}\w}{\tn{\La^{1/2}\w}}+\frac{\g_2^T\La_2^{1/2}\w}{\tn{\La^{1/2}\w}}
\end{align*}
\end{proof}
\begin{lemma}[Low-rank covariance] \label{low rank lem}Suppose positive semidefinite matrix $\bSi$ is of rank $r$. Then
\[
\omega_{\bSi}(\Tc)\leq \sqrt{r}.
\]
\end{lemma}
\begin{proof} Let $\bSi=\Ub\La\Ub^T$ where $\Ub\in\R^{p\times r}$ is unitary. Let $\tilde{\g}=\Ub^T\g$ and define the set $\tilde{\Tc}=\La^{1/2}\Ub^T\Tc\subset\R^r$.
\[
\sup_{\w\in\Tc}\frac{\g^T\bSi^{1/2}\w}{\tn{\bSi^{1/2}\w}}= \sup_{\tilde{\w}\in\tilde{\Tc}}\frac{\tilde{\g}^T\tilde{\w}}{\tn{\tilde{\w}}}\leq \sup_{\tilde{\w}\in\Bc^d}\frac{\tilde{\g}^T\tilde{\w}}{\tn{\tilde{\w}}}= \tn{\tilde{\g}}.
\]
Hence $\omega_{\bSi}(\Tc)\leq \E[\tn{\tilde{\g}}]\leq \sqrt{r}$.
\end{proof}
The following lemma follows from Sudakov-Fernique (see Exercise 7.2.13 of \cite{vershynin2018high}).
\begin{lemma}[Gaussian contraction principle] \label{contract}Let $\Tc\subset \R^p$, $(\phi_i(\cdot))_{i=1}^p$ be $1$-Lipschitz functions and $\g\sim\Nn(0,\Iden_p)$. Then
\[
\E[\sup_{\w\in\Tc}\sum_{i=1}^p g_i\phi_i(\w_i)]\leq \E[\sup_{\w\in\Tc}\g^T\w].
\] 
Let $\bSi\succeq\tilde{\bSi}$ be two positive semidefinite matrices with $0\preceq{\bSi}\preceq \tilde{\bSi}$. Then for $\g\sim\Nn(0,\Iden_p)$
\[
\E[\sup_{\w\in\Tc}\g^T\bSi^{1/2}\w]\leq \E[\sup_{\w\in\Tc}\g^T\tilde{\bSi}^{1/2}\w].
\] 
\end{lemma}
\begin{proof} Define the zero-mean Gaussian processes $X_{\w}=\g^T\bSi^{1/2}\w$ and $Y_{\w}=\g^T\bSi'^{1/2}\w$. Given $\vb,\w$, we verify Sudakov-Fernique condition as follows,
\begin{align}
\E(X_{\w}-X_{\vb})^2&=\E(\g^T\bSi^{1/2}(\w-\vb))^2=(\w-\vb)^T\bSi(\w-\vb)\\
&\leq (\w-\vb)^T\bSi'(\w-\vb)= \E(Y_{\w}-Y_{\vb})^2.
\end{align}
Hence $\E[\sup_{\w\in \Tc}X_{\w}]\leq \E[\sup_{\w\in \Tc}Y_{\w}]$.
\end{proof}
%\begin{proof} The proof of the latter part follows by writing $\g'=\Ub^T\g\sim\g$, $\Tc'=\tilde{\La}\Ub^T\Tc$ and setting $\phi_i(x)=\frac{\La_{ii}}{\tilde{\La}_{ii}}x$. With these note that
%\[
%\E[\sup_{\w\in\Tc}\g^T\tilde{\bSi}\w]=\E[\sup_{\w\in\Tc'}\g'^T\w]\geq \E[\sup_{\w\in\Tc'}\sum_{i=1}^p\g'_i\phi_i(\w_i)]= \E[\sup_{\w\in\Tc}\g^T{\bSi}\w]
%\]
%\end{proof}
\begin{lemma}[Gaussian Width and Condition Number] \label{condition lem}Let $\A\succeq 0$ and $\Iden_p\succeq \bSi_0\succeq \kappa^{-1}\Iden_p$. Let $\bSi=\bSi_0+\A$ and $\bSi'=\Iden_p+\A$. We have that
\[
\omega_{\bSi}(\Tc)\leq \sqrt{\kappa}\omega_{\bSi'}(\Tc).
\] 
\end{lemma}
\begin{proof} Observe that, for any $\w$%Suppose $\bSi'=\bSi+\la\ub\ub^T$.
\begin{align*}
\tn{\bSi^{1/2}\w}^2&=\w^T\bSi\w=\w^T\bSi_0\w+\w^T\A\w\geq \kappa^{-1}\tn{\w}^2+\w^T\A\w\\
&\geq \kappa^{-1}(\tn{\w}^2+\w^T\A\w)=\kappa^{-1}\tn{\bSi'^{1/2}\w}^2.
\end{align*}
Then, for $\h\sim\Nn(0,\Iden_p)$, applying Lemma \ref{contract}, it follows that
\begin{align}
\omega_{\bSi}(\Tc)&=\E[\sup_{\w\in\Tc}\frac{\w^T\bSi^{1/2}\h}{\tn{\bSi^{1/2}\w}}]\leq\sqrt{\kappa}\E[\sup_{\w\in\Tc}\frac{\w^T\bSi^{1/2}\h}{\tn{\bSi'^{1/2}\w}}]\\
&\leq \sqrt{\kappa}\E[\sup_{\w\in\Tc}\frac{\w^T\bSi'^{1/2}\h}{\tn{\bSi'^{1/2}\w}}]=\sqrt{\kappa}\omega_{\bSi'}(\Tc).
\end{align}
\end{proof}
