# Supplementary material for: Exploring Weight Importance and Hessian Bias in Model Pruning
Source: arXiv:2006.10903 source file (2020-06-19)
Supplement: Supplementary file 5 [file appendix_scaling.tex]

\section{Scale-Dependence of the Overparameterized Pseudo-inverse}\label{scale dep}
%\noindent {\bf{Pseudo-inverse change:}} 
The goal of this section is demonstrating the variability of feature importance in over-parameterized least-squares by studying the effect of feature scaling. 

%Our goal is finding a model $\bt$ with small test error i.e.~for a fresh sample $(\x,y)$, $\E[(y-\bt^T\x)^2]$ is small.
Suppose we are given a dataset $\y\in\R^n$ and $\X\in\R^{n\times p}$ and assume that $\X$ is full-rank. Clearly pseudo-inverse $\hat{\bt}=\X^\dagger \y$ is a common method for finding a model $\bt$ that can predict $\y$ given $\X$. Now, let $\La\in\R^{p\times p}$ be a diagonal matrix with nonnegative diagonal entries which will be used to scale our $p$ features as follows.

Let us consider a problem with labels $\y$ and scaled input features $\X\sqrt{\La}$. In this case, an alternative model that can predict $\y$ given unscaled $\X$ can be obtained by solving pseudo-inverse on the scaled problem $(\y,\X\sqrt{\La})$ and multiplying the solution by $\sqrt{\La}$ to account for the scaling. This model is given by
\[
\hat{\bt}_{\La}=\sqrt{\La}(\X\sqrt{\La})^\dagger \y.
\]
%Alternatively, one can estimate $\bt$ by solving the problem with labels $\y$ and inputs $\X\sqrt{\La}$. %Now  $\X$ is scaled with a diagonal matrix $\La^{1/2}$, we have the pair 
It is a simple exercise to show that if the problem is under-parameterized ($n\geq p$), $\hat{\bt}_{\La}$ is independent of scaling $\La$ and is always equal to the true pseudo-inverse $\hat\bt=\X^T(\X\X^T)^{-1}\y$. However if the problem is over-parameterized, $\hat{\bt}_{\La}$ has $\La$ dependence and is given by
\begin{align*}
\hat{\bt}_{\La}&=\sqrt{\La}(\X\sqrt{\La})^\dagger \y=\sqrt{\La}(\sqrt{\La}\X^T(\X\La\X^T)^{-1}\y)\\
&=\La\X^T(\X\La\X^T)^{-1}\y.
\end{align*}
Following this observation, we will show that as a feature weight increases (i.e.~diagonal entry of $\La$ associated to that feature), the model weight (the corresponding entry of $\hat{\bt}_{\La}$) increases as well. The following lemma summarizes this by focusing on scaling the first feature (without losing generality). 
\begin{lemma}[Feature scaling in linear regression] Suppose $p>n$. Let $\La=\text{diag}([\la~1~1~\dots~1])$. Given $\X,\y$ consider the scaled pseudo-inverse model defined as $\hat{\bt}_{\la}:=\hat{\bt}_{\La}$. Let $\x$ be the first column of $\X$. Suppose remaining $p-1$ columns of $\X$ have full row-rank and define their inverse gram matrix as $\Cb=(\X\X^T-\x\x^T)^{-1}$. The first entry of $\hat{\bt}_{\la}$ is given by
\[
\hat{\bt}_{\la,1}=\frac{\x^T\Cb\y}{\la^{-1}+\x^T\Cb\x}.
\]
\end{lemma}
As $\la$ increases from $0$ to $\infty$, $\hat{\bt}_{\la,1}$ moves from $0$ to $\frac{\x^T\Cb\y}{\x^T\Cb\x}$. Specifically, the model weight $|\hat{\bt}_{\la,1}|$ of the first feature is a strictly increasing function of $\la\geq 0$ whenever $\x^T\Cb\y\neq 0$.

\begin{proof}
%Let $\y=\X\eb_1$. We have $\hat\bt=\X^\dagger \y=\X^T(\X\X^T)^{-1}\y$. The solution of $\X\sqrt{\La}$ is given by . Then $\hat{\eb}_1=\La^{1/2}\hat\bt=\La\X^T(\X\La\X^T)^{-1}\y$.
%\[
%\X\La\X^T=\sum_{i=1}^p \la_i\x_i\x_i^T.
%\]
%In the extreme case of $n=1$, $\hat{\eb}_1$ is strictly increasing function of the entries of $\La$. What about matrix inversion lemma for more general case?
Set $\Cb=(\X_-\X_-^T)^{-1}$. Note that $\X\sqrt{\la}(\X\sqrt{\la})^T=\Cb^{-1}+\la\x\x^T$. Let us apply Matrix Inversion Lemma to obtain
\[
(\X\La \X^T)^{-1}=\Cb-(\la^{-1}+\x^T\Cb\x)^{-1}\Cb\x\x^T\Cb
\]
Hence
\[
(\X\La \X^T)^{-1}\y=(\Iden-(\la^{-1}+\x^T\Cb\x)^{-1}\Cb\x\x^T)\Cb\y.
\]
%\[
%\frac{\la_i x_i}{\sum_{i=1}^p \la_ix_i^2}
%\]
Consequently, the first entry of $\La\X^T(\X\La \X^T)^{-1}\y$ is given by
\begin{align*}
\hat{\bt}_{\la,1}&=\la\x^T(\Iden-(\la^{-1}+\x^T\Cb\x)^{-1}\Cb\x\x^T)\Cb\y\\
&=\la\x^T\Cb\y(1-\frac{\x^T\Cb\x}{\la^{-1}+\x^T\Cb\x})\\
&=\la\x^T\Cb\y(\frac{\la^{-1}}{\la^{-1}+\x^T\Cb\x})\\
&=\frac{\x^T\Cb\y}{\la^{-1}+\x^T\Cb\x}.
%\\&\la-\la(\la^{-1}+\x^T\Cb^{-1}\x)^{-1}\x^T\Cb^{-1}\x=\la(1-\frac{\alpha}{\la^{-1}+\alpha})=\frac{1}{\la^{-1}+\alpha}
\end{align*}
Note that $\lim_{\la\rightarrow 0}\hat{\bt}_{\la,1}=0$ and $\hat{\bt}_{\infty,1}=\frac{\x^T\Cb\y}{\x^T\Cb\x}$.
%Differentiating, we find that feature weight is a strictly increasing function of $\la$.
\end{proof}
