# Supplementary material for: Exploring Weight Importance and Hessian Bias in Model Pruning
Source: arXiv:2006.10903 source file (2020-06-19)
Supplement: Supplementary file 6 [file appendix_single.tex]

\section{Small Sample Complexity of Important Features}% in a Single Gradient Iteration}

%{Consider making this section for single index models}

In this section, we consider single index models and establish sample complexity bounds for selecting the most informative features. We will show that stronger features can be identified from fewer samples. Consider a dataset $(\x_i,y_i)_{i=1}^n$, where labels are generated by input samples $\x_i$ and a parameter $\bt$ via $y_i=\phi(\x_i^T\bt)$. Here $\phi$ is a possibly unknown and nonlinear link function (such as ReLU or sign function). Our interest is not recovering the exact model ($\bt$) but estimating the features which are most critical for the label prediction. For simplicity suppose $\x_i\distas\Nn(0,\La)$ where $\La$ is a diagonal matrix with diagonal values $\la_i$. In this setup, it is clear that the distribution before nonlinearity $\phi$ is given by
\[
\x_i^T\bt\distas \Nn(0,\sigma^2)\quad\text{where}\quad \sigma^2=\sum_{i=1}^n \theta_i^2\la_i.
\]
Setting $\bar{\bt}=\sqrt{\La}\bt$, the most important features for prediction are the locations of the largest entries of $\bar{\bt}$. This is because the largest entries of $\bar{\bt}$ are responsible for explaining most of the signal energy ($\x_i^T\bt$). The following result shows that features responsible for $\eps$ fraction of the signal energy can be identified from $\Omega(\eps^{-2})$ samples after a single gradient iteration. We remark that single-index models with sparsity constraints have been studied by multiple works including \cite{thrampoulidis2020generalized,plan2016high,plan2016generalized,oymak2017fast,ganti2015learning}. Unlike these works, result below focuses on feature selection for arbitrary (not necessarily sparse) model $\bt$.

\begin{lemma}[Single-index models] Consider a single index model as follows. Let $\x\sim \Nn(0,\La)$ where $\La$ is a diagonal matrix with entries $(\la_i)_{i=1}^p$. The label $y$ is obtained by $y=\phi(y_{lin})$ where $y_{lin}=\bt^T\x$. Generate dataset $(\x_i,y_i)_{i=1}^n \distas(\x,y)$. Set input energy $\xi=\E[y_{lin}^2]$ and let $S_{\eps}$ be the set of $\eps$ important features (energy-wise) defined as
\[
S_{\eps}=\{i\bgl \E[(x_i\theta_i)^2]\geq \eps\xi,~1\leq i\leq p\}.
\]
Set $\mu=\frac{\E[y_{lin}y]}{\xi}$ and $\alpha=\frac{\tsub{y-\mu y_{lin}}}{\sqrt{\xi}}$ and $t\geq 1$. If $\sqrt{n}\gtrsim \frac{t(\alpha/\mu+1)}{\delta\eps}$, then with probability $1-6p\exp(-tn)$, the largest $|S_{(1+\delta)\eps}|$ entries (in absolute value) of $\hat{\bt}=\mu^{-1}\text{diag}(\X^T\X)^{-1/2}\X^T\y$ is a subset of $S_{\eps}$.
\end{lemma}
Setting $\delta=1$, this result shows that the largest entries (first $|S_{2\eps}|$ of them) of the estimate $\hat{\bt}$ are all guaranteed to be $\eps$ important features of the problem. The sample complexity grows as $\eps^{-2}$ and depends on the properties of the nonlinear link function. Here $\mu$ quantifies the amount of linearity of the link function and $\alpha$ captures the nonlinearity. For typical link functions (such as ReLU), $\alpha/\mu$ is a constant.
 
\begin{proof}
Set $\bar{\x}=\La^{-1/2}\x\distas\Nn(0,\Iden)$, $\bar{\bt}=\La^{1/2}\bt$ and $\h=\frac{\La^{-1/2}\X^T\y}{n}$. Note that $\tn{\bar{\bt}}=\sqrt{\xi}$ and observe that
%\\{Make this argument for general covariance matrices?}
%\begin{align}
%\h=\frac{1}{n}\La^{1/2}\bar{\X}^T\X\bt=\frac{1}{n}\La^{1/2}\bar{\X}^T\bar{\X}\bar{\bt}.
%\end{align}
%\begin{align}
%\h&=\X^\dagger\y=\X^T(\X\X^T)^{-1}\y=\La^{1/2}\bar{\X}^T(\bar{\X}\La\bar{\X}^T)^{-1}\bar{\X}\bar{\bt}\\
%&=\X^\dagger\y=(\X^T\X)^{-1}\X^T\y=(\La^{1/2}\bar{\X}\bar{\X}^T\La^{1/2})^{-1}\La^{1/2}\bar{\X}^T\bar{\X}\bar{\bt}
%\end{align}
\begin{align}
\h&=\frac{\La^{-1/2}}{n}\sum_{i=1}^n y_i\x_i=\frac{\La^{-1/2}}{n}\sum_{i=1}^n \x_i\phi(\x_i^T\bt)=\frac{1}{n}\sum_{i=1}^n \xb_i\phi(\xb_i^T\bar{\bt})\\
&=\underbrace{\frac{1}{n}\sum_{i=1}^n \xb_i(\phi(\xb_i^T\bar{\bt})-\mu \xb_i^T\bar{\bt})}_{\h^n}+\mu\underbrace{\frac{1}{n} \sum_{i=1}^n \xb_i \xb_i^T\bar{\bt}}_{\h^l}.
\end{align}
Define $\tilde{\bt}=\bar{\bt}/\tn{\bar{\bt}}=\bar{\bt}/\sqrt{\xi}$. Let $\vb_i\distas \Nn(0,\Iden)$ and let $\xt_i=(\Iden-\tilde{\bt}\tilde{\bt}^T)\x_i+\tilde{\bt}\tilde{\bt}^T\vb_i\sim\Nn(0,\Iden)$. Observe that
\begin{align}
%((\Iden-\bt\bt^T)\xb_i +\bt\xb_i^T\bt)(\phi(\xb_i^T\bar{\bt})-\mu \xb_i^T\bar{\bt})=
\xb_i=\xt_i+\tilde{\bt}\tilde{\bt}^T(\xb_i-\vb_i)
\end{align}
As next step, the $j$th entry of $\h^l$ can be written as
\begin{align}
h_j^l&=\frac{1}{n}\sum_{i=1}^n \bar{x}_{i,j}\xb_i^T\bar{\bt}\\
&=\frac{1}{n}\sum_{i=1}^n(\bar{\theta}_j +\bar{\theta}_j (\bar{x}_{i,j}^2-1)+\bar{x}_{i,j}\xb_{i,\neq j}^T\bar{\bt}_{i,\neq j})
%=\sqrt{\la}_j\theta_j+\sum_{i=1}^n\sqrt{\la_i\la_j}\theta_i.
\end{align}
Now observe that $\E[\h]=\mu\E[\h^l]=\mu\bar{\bt}=\mu\sqrt{\La}\bt$. The zero-mean component can be bounded by noting
\[
\te{\bar{\theta}_j (\bar{x}_{i,j}^2-1)+\bar{x}_{i,j}\xb_{i,\neq j}^T\bar{\bt}_{i,\neq j}}\lesssim \tn{\bar{\bt}}=\sqrt{\xi}.
\] 
Applying subexponential concentration \cite{Vers} and union bound, with probability $1-2p\exp(-tn)$ all entries of $\h^l$ satisfies
\begin{align}
|h^l_j-\E[h^l_j]|\leq \frac{t\sqrt{\xi}}{\sqrt{n}}.\label{linear part}
\end{align}
The $j$th entry of $\h^n$ is bounded as
\begin{align}
\h^n&=\frac{1}{n}\sum_{i=1}^n \xb_i(\phi(\xb_i^T\bar{\bt})-\mu \xb_i^T\bar{\bt})\\
&=\frac{1}{n}\sum_{i=1}^n [(\xt_i+\tilde{\bt}\tilde{\bt}^T(\xb_i-\vb_i))(\phi(\xb_i^T\bar{\bt})-\mu \xb_i^T\bar{\bt})].
%&=\underbrace{\frac{1}{n}\sum_{i=1}^n \La^{1/2}[\xt_i(\phi(\xb_i^T\bar{\bt})-\mu \xb_i^T\bar{\bt})]}_{T^n_1}+\underbrace{\frac{1}{n}\sum_{i=1}^n \La^{1/2}[\tilde{\bt}\tilde{\bt}^T(\xb_i-\vb_i)(\phi(\xb_i^T\bar{\bt})-\mu \xb_i^T\bar{\bt})]}_{T^n_2}
\end{align}
Each entry of $\h^n$ can be written as 
\[
h^n_j=\frac{1}{n}\sum_{i=1}^n(\xt_{i,j}+\tilde{\bt}_j\tilde{\bt}^T(\xb_i-\vb_i))(\phi(\xb_i^T\bar{\bt})-\mu \xb_i^T\bar{\bt})
\]
Now observe that all terms above are zero-mean as $\xt,\vb$ is independent of $\xb_i^T\bar{\bt}$ and $\E[(\phi(y_{lin})-\mu y_{lin})y_{lin}]=0$. $\tsub{\phi(\xb_i^T\bar{\bt})-\mu \xb_i^T\bar{\bt}}\leq \alpha\sqrt{\xi}$. This implies that 
\[
\te{\tilde{\bt}_j\tilde{\bt}^T(\xb_i-\vb_i)(\phi(\xb_i^T\bar{\bt})-\mu \xb_i^T\bar{\bt})}\lesssim \alpha\sqrt{\xi}\quad,\quad \te{\xt_{i,j}(\phi(\xb_i^T\bar{\bt})-\mu \xb_i^T\bar{\bt})}\lesssim \alpha\sqrt{\xi}
\]
Hence, $h^n_j$ is sum of $n$ i.i.d.~zero-mean subexponential random variables. Applying subexponential concentration \cite{Vers}, with probability at least $1-2p\exp(-tn)$, for all $1\leq i\leq p$, we find that%$1-2\exp(-\frac{t^2n}{\alpha^2\xi^2}\wedge \frac{tn}{\alpha\xi})$
\begin{align}
|h^n_{j}|\lesssim \frac{t\alpha \sqrt{\xi}}{\sqrt{n}}= \frac{t\alpha\sqrt{\xi}}{\sqrt{n}}\label{nonlin part}
\end{align}
Combining \eqref{linear part} and \eqref{nonlin part}, we obtain that $\db=\h-\E[\h]=\h-\mu\bar{\bt}$ has entries bounded by
\[
\tin{\db}\leq \frac{t(\alpha+\mu)\sqrt{\xi}}{\sqrt{n}}.
\]
To proceed, consider $\h'=\text{diag}(\X^T\X)^{-1/2}\X^T\y=\text{diag}(\bar{\X}^T\bar{\X})^{-1/2}\La^{-1/2}\X^T\y$. We study the entrywise difference between $\h'$ and $\h$ which is given by
\[
\h'-\h= (\text{diag}(\frac{\bar{\X}^T\bar{\X}}{n})^{-1/2}-\Iden)\h.
\]
Using subexponential concentration yet another time, we have $\|\text{diag}(\frac{\bar{\X}^T\bar{\X}}{n})^{-1/2}-\Iden\|\lesssim t/\sqrt{n}$ with probability $1-2p\exp(-tn)$. Combining, we find that
\[
|h'_i-\mu\bar{\bt}_i|\lesssim  \frac{t(\alpha+\mu)\sqrt{\xi}+t\mu|\bar{\bt}_i|}{\sqrt{n}}\lesssim\frac{t(\alpha+\mu)\sqrt{\xi}}{\sqrt{n}} \iff |\mu^{-1}h'_i-\bar{\bt}_i|\lesssim  \frac{t(\alpha/\mu+1)\sqrt{\xi}}{\sqrt{n}}
\]
%which establishes the first claim. Next, we will show that most important features will be selected under sufficient spectral bias. First observe that if $n\geq \dots$, we have that
Next, observe that, whenever $n$ satisfies the advertised bound $n\gtrsim \frac{t^2(\alpha/\mu+1)^2}{\delta^2\eps^2}$, we have that
\begin{align}
|\mu^{-1}h'_i-\bar{\bt}_i|\leq \eps\delta \sqrt{\xi}/2.%\iff \mu\geq  \frac{t(\alpha+\mu)\sqrt{\xi}}{\sqrt{n}}\iff \frac{|\bar{\bt}_i|}{\sqrt{\xi}}\geq  \frac{t(\alpha/\mu+1)}{\sqrt{n}}
\end{align}
For $i\in S_{(1+\delta)\eps}=\supp{(1+\delta)\eps\sqrt{\xi}}{\bar{\bt}}$, this implies that $|\mu^{-1}h'_i|\geq (1+\delta/2)\eps\sqrt{\xi}$. In contrast, for $i\not\in  S_{\eps}=\supp{\eps\sqrt{\xi}}{\bar{\bt}}$, we have $|\mu^{-1}h'_i|< (1+\delta/2)\eps\sqrt{\xi}$. Combining this, we find that top $|\supp{(1+\delta)\eps\xi}{\bar{\bt}}|$ entries of $\mu^{-1}\h'$ is subset of $ \supp{\eps\xi}{\bar{\bt}}$.
%Specifically recall the definition of $\Gamma$. 
%We next bound the $T_1$ term which can be done similarly. This time, 
%Select most predictive features i.e. $\gamma$ fraction of the overall energy.
\end{proof}
%\[
%\La^{-1/2}\bSi^{1/2}-\Iden=\bar{\bSi}^{1/2}-\Iden???
%\]
%\[
%(\phi(\sum_ig_i)-\mu \sum_ig_i) g_1
%\]
%\subsection{Polyak}
